# Supplementary material for: AntEval: Evaluation of Social Interaction Competencies in LLM-Driven Agents
Source: arXiv:2401.06509 source file (2024-03-05)
Supplement: Supplementary file 1 [file supp.tex]

\appendix
\section{Appendix}
\label{sec:appendix}

\subsection{Details for Agent Interaction Framework} \label{settings}

\subsubsection{Introduction for TRPG and DND:}

Tabletop Role-Playing Games (TRPGs) represent a form of interactive and collaborative storytelling where players assume the roles of characters in a fictional setting. Governed by a set of rules and often mediated by a game master (GM) or dungeon master (DM), TRPGs facilitate the creation of narratives through player choices, character actions, and the outcomes of these actions as determined by game mechanics and dice rolls. These games emphasize creativity, teamwork, and strategic thinking, allowing players to explore diverse worlds, solve complex puzzles, and engage in combat with adversaries in a structured yet imaginative environment. The essence of TRPGs lies in their ability to blend narrative depth with player agency, fostering a unique storytelling experience that evolves with each session.

Dungeons \& Dragons (DND) stands as a quintessential example of TRPGs, pioneering many of the conventions and mechanics that have come to define the genre since its inception in 1974~\cite{gygax1974dungeons}. DND immerses players in a fantasy universe inspired by mythologies, folklore, and genre literature, where they create characters to embark on epic quests, battle fearsome monsters, and uncover vast treasures. The game is characterized by its complex rule system, which covers character creation, combat, magic, and progression, all orchestrated by the DM who guides the narrative and interprets the rules. DND's enduring popularity stems from its rich lore, extensive world-building, and the freedom it offers players to craft their own adventures within its expansive multiverse. As a cornerstone of TRPG culture, DND has not only entertained generations of gamers but also influenced a wide array of media, game design, and even academic fields, making it a seminal work in the landscape of interactive storytelling.

\subsubsection{Settings for Character Generation}
\begin{figure*}[!t]
	\centering
	\includegraphics[width=\textwidth]{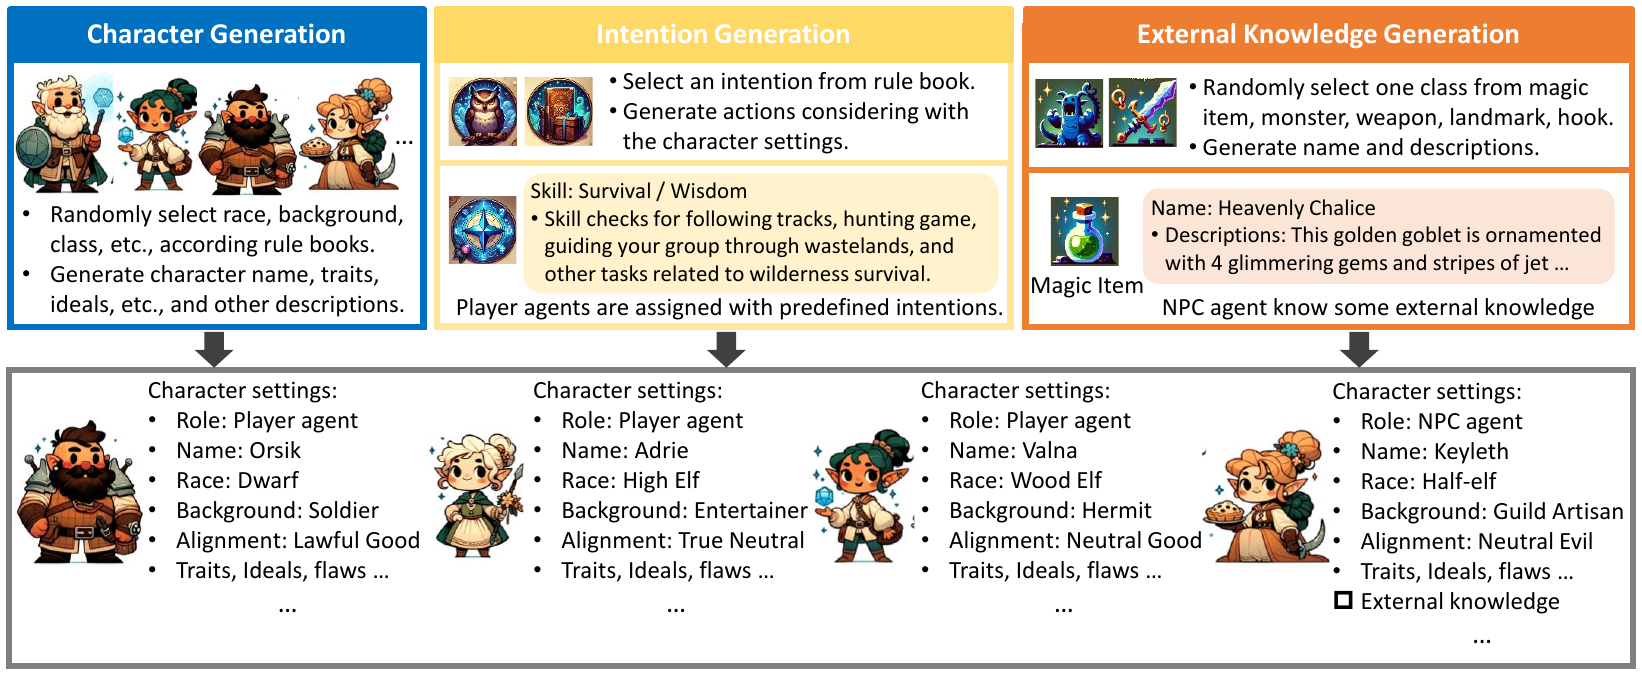}
	\caption{Overview of character generation.}
	\label{fig::supp_gen_char}
\end{figure*}

\textbf{Character settings:}
We start by constructing a character following DND rules, focusing on essential attributes such as name, race, background, class, alignment, personality, ideals, bonds, flaws, and appearance. Specifically, race, background, class and alignment are pre-defined categories in DND rules, as shown in Fig~\ref{fig::supp_gen_char}. 

In detail, we follow the instructions in~\cite{gygax1974dungeons}, which show how to create a DND character step-by-step. To reduce the complexity, we remove the number system of DND rules and only keep the descriptions and settings. We also remove the equipment settings for characters. Then, following~\cite{gygax1974dungeons}, creating a character in DND involves a series of choices that together form a vivid, multi-dimensional persona players will explore and develop throughout their adventures. We provide the descriptions of each component used in our work involved in character creation:

\begin{itemize}
  \item Name: The name of a DND character serves as the first introduction to their identity, echoing the cultures, languages, and traditions of their in-game universe. It might hint at their heritage, the lands they hail from, or the values their society holds dear. A well-chosen name sets the tone for the character's backstory, their interactions, and how they are perceived by others in the game world, weaving a rich tapestry of mystery, power, or destiny around them.
  \item Race: Race in DND goes beyond mere physical appearance; it encompasses a character's biological heritage, imbuing them with specific traits, abilities, and predispositions. From the sturdy and industrious dwarves to the graceful and arcane elves, each race brings its unique characteristics, history, and worldview to the character's development. This choice influences the character's physical attributes, languages spoken, and special skills, offering a foundation upon which their personality and abilities are built.
  \item Background: A character's background provides a glimpse into their life before the adventuring begins, shaping their skills, proficiencies, and traits. Whether a noble with a life of luxury, a soldier hardened by war, or a rogue with a mysterious past, the background adds depth to the character's story, influencing their motivations, fears, and dreams. It serves as a narrative tool that explains how they came to be who they are and what drives them forward.
  \item Class: The class represents the character's profession or vocation, defining their skills, abilities, and approach to challenges. From the spell-wielding wizards and clerics channeling divine power to the stealthy rogues and valiant fighters, the class dictates the role the character will play in the party and how they contribute to their collective success. It shapes their journey, the challenges they'll face, and the paths they'll choose.
  \item Alignment: Alignment is the moral and ethical compass that guides a character's decisions and interactions. Ranging from lawful good, through true neutral, to chaotic evil, alignment reflects the character's beliefs, values, and personality. It influences how they respond to moral dilemmas, interact with other characters, and perceive the world around them, adding complexity and conflict to the narrative.
  \item Personality: A character's personality breathes life into the stats and facts, encapsulating their hopes, fears, quirks, and mannerisms. It's what makes them memorable and relatable, driving their reactions to success, failure, and the myriad experiences they'll encounter. A well-crafted personality allows for growth and change, reflecting the character's journey through the game.
  \item Ideals: Ideals are the core beliefs and principles that motivate a character's actions and decisions. They stem from the character's background, culture, and personal experiences, guiding them toward their goals. Whether it's the pursuit of justice, freedom, knowledge, or power, ideals help define what the character stands for and what they're willing to fight for.
  \item Bonds: Bonds represent the character's connections to people, places, and events in the world. These could be family ties, friendships, a vow, or a cherished memory, grounding the character in the game's setting and driving many of their choices. Bonds add emotional depth and can serve as powerful motivators or sources of conflict within the story.
  \item Flaws: Flaws are the imperfections and weaknesses that make a character human (or elf, dwarf, etc.). They could be a fear, a vice, an enemy, or a secret that haunts them. Flaws create vulnerability and complexity, making the character more interesting and relatable, and providing opportunities for character development and dramatic tension.
  \item Appearance: A character's appearance includes their physical features, attire, and personal style, contributing to their first impression and how they navigate their social environment. It can reflect their background, class, and personal history—armor bearing the scars of battle, robes adorned with arcane symbols, or the refined attire of a noble. Appearance sets the stage for initial interactions and can influence how characters are perceived and treated by others in the game world.
\end{itemize}

Each of these elements combines to create a richly detailed and cohesive character, ready to embark on epic adventures and forge their destiny in the world of DND. We randomly select these attributes to construct a character. Then, we use LLMs to generate character names and detailed descriptions involving personality, ideals, bonds, flaws, and appearance, taking into acount the selected pre-defined attributes.  

\textbf{Settings generation: }
In the realm of character creation for a fantasy setting, there are various categories to define a character's attributes and background. These categories include race, background, class, and alignment, each with its own set of options to choose from.

Starting with race, characters can belong to one of several races, each with distinct subraces. For example, Dragonborn characters can be of various types, reflecting the lineage of different dragons like Black, Blue, Brass, Bronze, Copper, Gold, Green, Red, Silver, and White Dragonborn. Dwarves can be classified as Hill Dwarves or Mountain Dwarves, while Elves have subraces such as High Elves, Wood Elves, and Dark Elves (Drow). Gnomes can be Forest or Rock Gnomes. Other races include Half-Elves, Half-Orcs, and Halflings, with Halflings further divided into Lightfoot and Stout Halflings. Humans have a wide range of ethnicities, including Calishite, Chondathan, Damaran, Illuskan, Mulan, Rashemi, Shou, Tethyrian, and Turami. Finally, there are Tieflings, which represent those with a demonic heritage.

Moving on to background, characters come from diverse histories that influence their skills and professions. These backgrounds include Acolyte, Charlatan, Criminal, Entertainer, Folk Hero, Gladiator, Guild Artisan, Guild Merchant, Hermit, Knight, Noble, Outlander, Pirate, Sage, Sailor, Soldier, Spy, and Urchin. Each background provides a unique backstory and set of skills that enrich the character's role in the fantasy world.

Regarding class, characters can adopt various roles based on their skills and abilities. The options available are Barbarian, Bard, Cleric, Druid, Fighter, Monk, Paladin, Ranger, Rogue, Sorcerer, Warlock, and Wizard. Each class has its own strengths, weaknesses, and magical abilities that define the character's role in adventures and combat.

Lastly, alignment describes the moral and ethical stance of characters, ranging from good to evil and lawful to chaotic. The alignments are Lawful Good, Neutral Good, Chaotic Good, Lawful Neutral, Neutral (True Neutral), Chaotic Neutral, Lawful Evil, Neutral Evil, and Chaotic Evil. This spectrum allows for complex character personalities and moral choices.

Together, these categories provide a comprehensive framework for creating rich and varied characters in a fantasy setting, allowing for endless possibilities in storytelling and role-playing.

\textbf{Generation prompts:}
We first use settings randomly selected above as the basic information for construting the character, which is: 
\textit{Your race is Human (Illuskan). You class is Bard. Your alignment is Lawful Good. Your background is Gladiator.}

Building upon the foundational settings described earlier, we devised prompts to guide GPT-4 in generating additional character settings. These prompts are as follows:
\begin{itemize}
\item For name generation: 
\textit{According following character informatoin, `Your race is Human (Illuskan). You class is Bard. Your alignment is Lawful Good. Your background is Gladiator.' Write a character name to play a DND game.}
\item For personality generation: 
\textit{According following character informatoin, `Your race is Human (Illuskan). You class is Bard. Your alignment is Lawful Good. Your background is Gladiator.' write a character personality. For example: He walk his own path, regardless of how others criticize it. }
\item For ideals generation: 
\textit{According following character informatoin, `Your race is Human (Illuskan). You class is Bard. Your alignment is Lawful Good. Your background is Gladiator.' write a character ideals. For example: Helping others is the most important thing in the world. }
\item For bounds generation: 
\textit{According following character informatoin, `Your race is Human (Illuskan). You class is Bard. Your alignment is Lawful Good. Your background is Gladiator.' write a character bounds. For example: As a child, his twin sacrificed himself to a devil so that he may live, and now haunts his dreams with a motive he has yet to discern.}
\item For flaws generation: 
\textit{According following character informatoin, `Your race is Human (Illuskan). You class is Bard. Your alignment is Lawful Good. Your background is Gladiator.' write a character flaws. For example: He is quick to assume that someone is trying to cheat him. }
\item For appearance generation: 
\textit{According following character informatoin, `Your race is Human (Illuskan). You class is Bard. Your alignment is Lawful Good. Your background is Gladiator.' write a character appearance. For example: A white skinned woman with brown eyes, hollow cheeks, fine eyebrows, large lips and small ears. She has fine, dark brown hair, seems unassuming, has piercings in four places, usually wears a specific jumper, and she has a large boil on her face. She is carrying a small item.  }
\end{itemize}

\textbf{Character generation examples:}

Here is an example for the character description: 

\textit{You are Luna Silverstone, a NPC in a DND game, and you need to act following your own personality and should not cater to other characters' demands. Your race is Human (Illuskan). Your class is Bard. Your alignment is Lawful Good. Your background is `Gladiator'. Your personality is `This character is a charismatic and brave individual, with a heart full of compassion and a desire to uphold virtue and morality. Despite his background as a gladiator, he wields his verbal wits just as fiercely as any weapon. He can often be found using his bardic skills to encourage and motivate his allies, or charming his way out of potentially hazardous situations. His dutiful adherence to the law and innate goodness shine through in all of his decisions, regularly placing the needs of others before his own. He has a deep respect for rules and order and uses his charisma and conviction to inspire others to also seek righteousness and justice. He is fearless when it comes to standing up for what he believes in and is unwavering in his pursuit of fairness and equality. His inherent moral compass is guided by a profound sense of idealism and honor. Yet, his gladiatorial past reminds him of the harsh realities of the world, creating a delicate balance between his ideals and his pragmatism. Overall, he is a beacon of hope, righteousness, and moral integrity in a world that often needs it.'}

\textit{Your ideals are `As an Illuskan Bard who prevails as a gladiator, this character values discipline, honor, and courage. They believe in the power of a structured life, ruled by laws and fairness. Their ideal is the mantra of `Victory with Valor,' meaning they strive to win their battles, but not at the cost of their morals and ethics. They believe in a fair fight and despise cheating or unlawful actions. They see the art of music and storytelling as a vital tool to unite people, uplift spirits, and inspire strength. They hold high respect for skilled, honorable warriors and look down on those who use trickery or deceit to get ahead. They view life as a battlefield, where each day brings forth new challenges that need to be faced with bravery and resilience.'}

\textit{Your bonds are `Born under the harsh and frigid skies of the Frozenfar, our Illuskan Human was not always a gladiator by choice or a bard by passion, but rather by an unyielding pull from the gusts of destiny. Resilient in character and strong in physique, he has fought countless battles not only in the great arenas of the land but also in the depths of his soul and the strings of his lute. His imposing stature and battle-scars may count numerous tales of struggle and hard-won triumph, yet beneath the toughened exterior dwells a spirit rendered tender by the poignant melodies that fill his lonely nights. Raised in a family steeped in old traditions and the law of the land, his alignment is Lawful Good- a natural outcome shaped by the principles he witnessed and wise words he absorbed. Unyielding and steadfast, he pursues justice and fairness, standing unwavered against the odds, and often, his own demons. His moral compass, marked invariably towards 'good', he constantly aims to contribute to the society that recognized his strength not as a threat but a means of entertainment and protection.}

\textit{Reflecting his tumultuous yet thrilling journey, his music is diverse- echoing the raw cries of combat one moment and soothing the tired hearts with peaceful harmonies the next. With each strum of his lute, he recalls the weapons clashing, the eruptive applause from the stands, and the taste of victory- igniting the listeners' imaginations, taking them with him on his chronicles, and enkindling within them a flame of adventurous spirit.}

\textit{Haunted by the memories and dreams of his sibling's sacrificial act, however, he battles internal turmoils that little understand. His twin brother, who preferred the pen to the sword, traded his life for his at a crucial juncture. This mysterious act has left an indelible mark on the battle-weary gladiator, the looming shadow of his brother's sacrifice frequently visiting him in his dreams, and in his quiet tunes. The motive behind his brother's selfless act remains obscured, lending an undercurrent of mystery and conflict to his compelling character.}

\textit{Beneath the roars of his Gladiator past, the lyrical whispers of his Bard present, and the spectral echoes of familial sacrifice, rumbles a spirit of valor and kindness, ready to fight his fate with a sword in one hand and harmonies in another. The rhythm of his journey continues, resonating within himself, his music, and the legacy he bears.}

\textit{Your flaws are `Despite his Lawful Good alignment, he tends to be overly judgmental and harsh towards people who do not follow the rules as strictly as he does.'}

\textit{You know something about `The Valorous Arena. This ancient battleground was a platform for grand battles and deadly duels where gladiators fought with bravery, valor, and honor. Legend says it was enchanted by the famous bard and hero from the Illuskan tribe, turning it into a site of victory for the righteous and doom for the evil. Known for its storied history and spectral aura, this fallen coliseum both excites and terrifies you. As a gladiator, you have experienced the bloodshed in the arenas, but never something with so much legend and supernatural energy. The Valorous Arena's tales of triumph and tragedy inspire your bardic melodies, though its history hints at an uncanny mystery that you, being lawful good, are driven to unravel for the sake of justice.'}

\subsubsection{Settings for Interaction Generation}

\textbf{External knowledge settings:}
To assess informativeness, we endow NPCs with exclusive knowledge that player agents lack. This external knowledge encompasses five categories: magic items, weapons, landmarks, monsters, and adventure hooks. We use GPT-4 model to generate both the names and descriptions of these elements.

Specifically, in the sprawling, fantastical realms of DND, the setting is brought to life not just by the characters who inhabit it, but also by the myriad of objects, creatures, and mysteries that populate its landscape. We provide the descriptions of each component used in our work involved in external knowledge generation:

\begin{itemize}
\item Magic Items: 
Magic items in DND are artifacts imbued with arcane power, ranging from simple potions and enchanted weapons to legendary relics that hold the keys to immense power or dire consequences. Each item comes with its own lore, discovered through ancient texts, long-forgotten ruins, or the tales of those who once wielded them. These items can turn the tide of battle, unlock secrets, or curse those who use them without caution. The discovery of a magic item is not just a boon to a character's abilities but a doorway to new adventures, dangers, and stories.

\item Weapons: 
Weapons in DND are not merely tools of combat but symbols of the characters who wield them, reflecting their skills, heritage, and personal stories. From the elven longbow, crafted with the wood of ancient forests, to the dwarven axe, forged in the heart of a mountain under the watch of the god of smithing, each weapon carries the history of its making and use. Whether it's a simple dagger with a hidden mechanism or a sword that glows in the presence of orcs, weapons add a layer of strategy, personality, and narrative to the game.

\item Landmarks: 
Landmarks within the DND universe serve as beacons of adventure, mystery, and history. They can be towering castles haunted by the ghosts of a fallen dynasty, ancient trees where druids convene under the moonlight, or even a city floating in the sky, accessible only by those who know its secrets. These landmarks are not just points on a map but pivotal locations that drive the story, host epic battles, and uncover hidden truths. They anchor the world in a sense of place and history, offering gateways to other realms, treasures, or cataclysmic events.

\item Monsters: 
Monsters in DND are as varied as they are terrifying, ranging from the minions of the underworld to legendary beasts that threaten entire kingdoms. They embody the challenges and dangers of the world, each with its own lore, motivations, and weaknesses. Encounters with monsters are not just combat challenges but opportunities for storytelling, revealing the history of the land, the corruption of power, or the balance of the natural world. From dragons hoarding ancient treasures to undead armies ravaging the countryside, monsters are central to the drama and tension of the game.

\item Adventure Hooks: 
Adventure hooks are the narrative seeds from which campaigns grow, offering players a doorway into the mysteries and quests of the DND world. These hooks might be a call for help from a village under siege, a mysterious artifact that whispers in dreams, or an ancient prophecy that points to the players as its key figures. Adventure hooks draw characters into the heart of the story, challenging them to make choices that will shape their path, allies, and enemies. They are the invitation to adventure, promising untold dangers, rewards, and the chance to write their own legends.

\end{itemize}

In all, these elements create a rich, dynamic world that thrives on the imagination and decisions of its players, making every DND game a unique journey into the unknown.

\textbf{Generation prompts:}
The prompts we used to prompt GPT-4 to generate External knowledge are as follow: 

\begin{itemize}
\item For magic item generation: 
\textit{Write an magic item for the adventure and some corresponding descriptions. This is an item that you cherish greatly and you hope to be able to retrieve it. Moreover, this is an item that you acquired by chance, and you hope to be able to use it more effectively. For example \textbackslash n item: \{Eye of the Bookwurm. This small, glass sphere is enchanted with weak divination magics to help you find specific words or phrases in writing. It has a stylized iris etched into the glass. You can use a bonus action to speak the eye's command word aloud, followed by the word or phrase you're searching for. The word or phrase magically appears and floats within the sphere. By holding the eye in a free hand, your vision becomes magically enhanced to subconsciously highlight the word or phrase you searched for in a green light wherever you see it. Once you've used the eye's ability for the first time, you can change the word or phrase as many times as you like for the next hour, after which the item can't be used again until the following dawn.\}\textbackslash n }

\item For weapon generation: 
\textit{Write an weapon for the adventure and some corresponding descriptions. This is a powerful weapon that you hope to find. Moreover, this is a weapon you have just acquired, and you hope to use it in your adventures. For example \textbackslash n weapon: \{Candleflame Bow. Description: Wrought from metal in the likeness of a brazier, this ranged weapon's grip has been covered in wax and has a simple candle positioned in front of where the arrow or bolt is fired from. The candle is magic and never runs out of wax, nor can it be removed from the weapon. You can use a bonus action to speak the weapon's command word to cause the candle to light itself, shedding bright light in a 15-foot radius and dim light for an additional 15 feet while it's ablaze. While the candle is lit, this magic weapon deals an extra 2 fire damage to any target it hits with a ranged attack. The candle's flame lasts until you use a bonus action to speak the command word again or until you drop or stow the weapon. If you roll the same number on both d20s when you make a ranged attack roll with advantage or disadvantage using this weapon while its candle is lit, the ammunition becomes wreathed in a conflagration of uncontrollable flames. The arrow or bolt flies toward the target and explodes, destroying the ammunition and dealing 4d6 fire damage to the target on a hit (instead of the attack's normal damage), or half as much damage if the result of the attack roll was less than the target's AC. This fire ignites flammable objects within 5 feet of the target that aren't being worn or carried. This property can't be used again until the next dawn.\}\textbackslash n }

\item For landmark generation: 
\textit{Write an landmark for the adventure and some corresponding descriptions. This is a locally well-known spot that you hope to find someone to explore with. You have learned that this place is often the site of strange occurrences, and you are very curious about it. You know that there are terrifying monsters at this location, and you would dissuade others from approaching it. You are very familiar with this location, and you can offer your services for a fee to guide people there. For example \textbackslash n Landmark: \{Circle of Covens. The witches of old gathered here. Newer generations of wicca have tried to understand its secrets, but any who attempt to gather here suffer a terrible curse.\}\textbackslash n }

\item For monster generation: 
\textit{Write an monster for the adventure and some corresponding descriptions. You encountered this monster in a previous adventure, and you hope to challenge and defeat it once more. Your family was attacked by this kind of monster, and you hope to completely eradicate this type of creature. You are very interested in this kind of monster, and you hope to conduct a detailed investigation of it. You have learned that parts of this monster\'s body can be used to cure your friend, and you hope to be able to hunt it. For example \textbackslash n monster: \{Circle Gray Bat. Lighting-gazing. Hard to predict. Has a gruesome magnolia hue. Likely causes insanity: Victim incessantly hums.\}\textbackslash n }

\item For hook generation, we first produce a brief magic item description and then fill in the prompt for hook generation. For example, the item description is: \textit{The Withered Gates. This intimidating structure of blackened stone and embedded bones stands at the entrance of the treacherous}. Then, the hook generation prompt is: 
\textit{write a hook for the item in the stroy. Description for the item: The Withered Gates. This intimidating structure of blackened stone and embedded bones stands at the entrance of the treacherous. You are willing to chat with others and share some gossip. For example \textbackslash n hook: Most people believe the treasure is real, while Drangor Lesley does not.\}\textbackslash n } 

\end{itemize}

\textbf{External knowledge examples:}

This is an example for generating a external knowledge, which is a monster description: 
\textit{Stonebound Mire Troll. Living in the thick of the marshes. Evil intentions hidden behind a facade of stone. Possesses a ferocious stamina. Enveloped in a bristly vine-green hue. Its gnarly visage incites blindness. Your family's homestead nestled in foothills was ravaged by this ominous monster. Your relatives spoken stories of their terrifying encounter with the formidable Stonebound Mire Troll were passed down to you. It is a creature not to be taken lightly. The treacherous beast appeared normal, blending with common boulders due to its rocky skin. But its inherent malevolence had spread a devastating curse blinding your ancestors. This haunting tale of the Stonebound Mire Troll's destruction has triggered an innate rage within you, sparking your journey as a Barbarian to slay this troll and safeguard your homeland. Your sole mission is to wipe this beast from the face of the earth, thus restoring peace and tranquility to your homeland.}

\subsection{Skill Check in DND and Intention in Interaction}

The skill check mechanism in Tabletop Role-Playing Games (TRPGs) is a fundamental system that quantifies and resolves the actions of characters within the game's narrative framework. This mechanism is adept at encompassing a broad spectrum of player behaviors, from physical feats and combat maneuvers to social interactions and intellectual challenges. The versatility of skill checks lies in their ability to translate the diverse and often complex intentions of players into measurable outcomes within the game's world.

At the heart of the skill check mechanism is the principle that every action, whether it's climbing a cliff, deceiving a guard, or researching ancient lore, can be represented by a combination of a character's abilities and the inherent difficulty of the task. This is achieved through the character's skill proficiencies, which are numerical representations of their training, experience, and innate talents in specific domains, such as stealth, persuasion, or arcana. When a player declares an action, they roll a die (typically a d20 in many TRPG systems) and add relevant modifiers based on their character's proficiency in the skill related to that action. The total is then compared against a difficulty class (DC), determined by the game master (GM), which represents how hard the task is to accomplish.

One of the reasons skill checks can describe most behaviors of players in the game is their inherent flexibility and adaptability. The system is designed to accommodate a wide range of actions and outcomes, allowing for creative problem-solving and unexpected strategies. Players are encouraged to think beyond the confines of predefined abilities or spells, using their skills in innovative ways to overcome obstacles. This not only enhances player agency but also enriches the storytelling process, as the outcome of skill checks can lead to narrative twists, character development, and dynamic interactions with the game world.

Moreover, skill checks serve as a bridge between the abstract decisions of players and the concrete realities of their characters' capabilities and the game's setting. They provide a structured yet fluid framework for translating the imaginative aspirations of players into in-game actions and consequences. This translation process ensures that player behavior is grounded in the game's mechanics and the fictional consistency of the world, fostering a sense of immersion and realism.

In essence, the skill check mechanism is a versatile tool that captures the breadth of player behavior by offering a systematic way to resolve actions, from the mundane to the extraordinary. It allows TRPGs to model an expansive range of activities and interactions, making it a key driver of player engagement, narrative depth, and the overall gaming experience. Through skill checks, players can fully inhabit their characters, exploring the limits of their abilities and the boundless possibilities of the game world.

In our work, we adopt skill check labels from game logs as annotations to represent intentions, streamlining the system by focusing solely on skill names and omitting numerical values and the rolling process. Specifically, we reference skills defined in the Dungeons and Dragons 5th Edition (DND 5E) rules~\cite{gygax1974dungeons}. In DND 5E, skills represent crucial abilities that enable characters to undertake particular actions or activities. Each skill correlates with a primary character attribute: Strength, Dexterity, Constitution, Intelligence, Wisdom, or Charisma. Additionally, although not classified as a skill, Initiative is a crucial mechanic tied to Dexterity. We provide a summary of each skill along with its related attribute as outlined in the DND 5E rules.

\begin{itemize}

\item Strength
\begin{itemize}
    \item Strength: This attribute measures bodily power, athletic training, and the extent to which you can exert raw physical force.
    \item Athletics: This skill covers difficult situations you encounter while climbing, jumping, or swimming. Athletics checks are made when you attempt to scale a cliff, jump over a chasm, or stay afloat in treacherous waters.
\end{itemize}

\item Dexterity
\begin{itemize}
    \item Dexterity: This attribute measures agility, reflexes, and balance.
    \item Acrobatics: This skill is used when you attempt to stay on your feet in a tricky situation, such as when you're trying to run across a sheet of ice, balance on a tightrope, or perform acrobatic stunts.
    \item Sleight of Hand: This skill is about performing tasks that require a delicate touch, like pickpocketing, concealing an object on your person, or manipulating a small device.
    \item Stealth: When you attempt to conceal yourself from enemies, slink past guards, slip away without being noticed, or sneak up on someone, you make a Stealth check.
\end{itemize}

\item Constitution
\begin{itemize}
    \item Constitution: Reflects your health and stamina. Constitution checks are not common and do not cover specific skills, but they might be tied to checks to endure harsh conditions or stave off disease.
\end{itemize}

\item Intelligence
\begin{itemize}
    \item Intelligence: This attribute measures mental acuity, accuracy of recall, and the ability to reason.
    \item Arcana: This skill is used when you recall knowledge about spells, magic items, eldritch symbols, magical traditions, the planes of existence, and the inhabitants of those planes.
    \item History: Your ability to recall lore about historical events, legendary people, ancient kingdoms, past disputes, recent wars, and lost civilizations.
    \item Investigation: When you look around for clues and make deductions based on those clues. It might be searching for a hidden object, deducing the location of a secret door, or deciphering an ancient riddle.
    \item Nature: This skill relates to recalling knowledge about terrain, plants and animals, the weather, and natural cycles.
    \item Religion: Your ability to recall knowledge about deities, rites and prayers, religious hierarchies, holy symbols, and the practices of secret cults.
\end{itemize}

\item Wisdom
\begin{itemize}
    \item Wisdom: This attribute reflects how attuned you are to the world around you and represents perceptiveness and intuition.
    \item Animal Handling: When you try to calm a domesticated animal, keep a mount from getting spooked, or intuit an animal's intentions.
    \item Insight: Used to determine the true intentions of a creature, such as when searching out a lie or predicting someone's next move.
    \item Medicine: This skill lets you try to stabilize a dying companion or diagnose an illness.
    \item Perception: Your ability to spot, hear, or otherwise detect the presence of something. It measures your general awareness of your surroundings and the keenness of your senses.
    \item Survival: This skill is used to follow tracks, hunt wild game, guide your group through frozen wastelands, identify signs that owlbears live nearby, predict the weather, or avoid quicksand and other natural hazards.
\end{itemize}

\item Charisma
\begin{itemize}
    \item Charisma: Measures your ability to interact effectively with others. It includes such factors as confidence and eloquence, and it can represent a charming or commanding personality.
    \item Deception: Your ability to convincingly hide the truth, whether you're trying to disguise your intentions or mask the truth with lies.
    \item Intimidation: When you attempt to influence someone through overt threats, hostile actions, and physical violence.
    \item Performance: Your ability to delight an audience with music, dance, acting, storytelling, or some other form of entertainment.
    \item Persuasion: When you attempt to influence someone or a group of people with tact, social graces, or good nature.
\end{itemize}

\item Initiative
\begin{itemize}
    \item Initiative: Not a skill, but a mechanic that determines the order of turns in combat. Initiative is an ability check using your Dexterity modifier. It reflects quick reflexes and the ability to react swiftly to danger.
\end{itemize}

\end{itemize}

\subsection{Statistics of Training Data for IEG}
statistically, the real interaction data comprises $838$ logs, sourced from game logs of human players as detailed in~\cite{liang2023tachikuma}. We utilize $661$ of these logs for fine-tuning our models, while the remaining $177$ logs serve as the evaluation dataset. The real data selected for fine-tuning encompasses a total of $24,615$ interactions. Comparatively, we generate agent interactions across $600$ different sessions, each consisting of $30$ turns, to reduce biases from size differences between generated data and real data.

% \textbf{Number of key points}
% Different LLMs are employed as summarization models to summarize the agents' responses. These summaries are then compared with predefined ground truths to determine the number of matching key points and calculate a match score. We present both the average precision and variance in our experiments. To account for variability in summarization and prediction, each interaction set undergoes $5$ times of prediction and evaluation. The average precision of matching key points and the variance in these precisions are then calculated.
% \begin{table}[]
% 	\begin{center}
% 	\resizebox{  \columnwidth}{!}
%       {
%         \begin{tabular}{|l|l|l|l|l|}
%         \hline
%         Number of key points & \multicolumn{1}{c|}{$k=1$} & \multicolumn{1}{c|}{$k=5$} & \multicolumn{1}{c|}{$k=10$} & \multicolumn{1}{c|}{$k=20$} \\ \hline \hline 
%         Average Precision    &                        &                        &                         &                         \\ \hline
%         \end{tabular}
%       }
%      \end{center}
%     \caption{Ablation for the number of key points.  }
%     \label{table::tab_kp_ablation}
% \end{table}
\subsection{Evaluation of Summarization Models}
\begin{table}[]
	\begin{center}
	\resizebox{0.8\columnwidth}{!}
      {
        \begin{tabular}{|l|cc|}
        \hline
        \multicolumn{1}{|c|}{\multirow{2}{*}{Summarization Model}} & \multicolumn{2}{c|}{Evaluation Model}                     \\ \cline{2-3} 
        \multicolumn{1}{|c|}{}                                     & \multicolumn{1}{c|}{GPT-3.5} & \multicolumn{1}{c|}{GPT-4} \\ \hline \hline 
        GPT-3.5                                                    & \multicolumn{1}{c|}{39.22}   & 36.80                      \\ \hline
        GPT-4                                                      & \multicolumn{1}{c|}{55.93}   & 60.40                      \\ \hline
        \end{tabular}
     }
     \end{center}
    \caption{Comparison for the mean precision of key point prediction in AntEval. }
    \label{table::tab_avg_prec}
\end{table}

In our informativeness evaluation, we compare the GPT-3.5 and GPT-4 models. These models act as characters in DND, generating interactions and responding to queries about the information they gather during these interactions. A summarization model is then used to summarize the responses into key points for comparison with predefined ground truths. We report the average precision of these key points in Tab~\ref{table::tab_avg_prec}. Our experiments show that the performance gap between the GPT-3.5 and GPT-4 models is modest. When GPT-3.5 serves as the summarization model, it slightly outperforms GPT-4 by $2.42\%$. In contrast, when GPT-4 is used as the summarization model, it outperforms GPT-3.5 by $4.47\%$, which is also relatively modest. These results lead to two key observations:
1). Improving informativeness in agent interactions is challenging. All models, despite their advanced capabilities, struggle in this framework. Social interactions, which are typically more straightforward for humans and do not require extensive logical analysis or reasoning, pose a significant challenge to LLMs, highlighting their limitations in social interaction processing and pointing to areas for improvement.
2). The performance gap between models of different capacities is not significant. Although GPT-4 is more advanced than GPT-3.5, it does not consistently outperform in every scenario. This suggests that current LLMs might not be fully optimized for long-context interactions and may lack the necessary capabilities for effective and informative expression. Interactions often tend to be conservative and repetitive, lacking the depth and richness of real-life human communication.

Furthermore, the choice of the summarization model plays a crucial role. Summarizing with GPT-4 significantly improves performance compared to using GPT-3.5. This implies that while agents might be conveying useful information, the ability of the summarization model to capture these nuances varies, reflecting the different semantic understanding capabilities of LLMs. The notable performance improvements of $16.71\%$ and $23.60\%$, respectively, when using GPT-4 as opposed to GPT-3.5 as a summarization model, underscore the importance of enhancing LLMs' comprehension abilities. More sophisticated LLMs, proficient in interpreting human semantics, could potentially lead to better performance in summarizing key points, thereby increasing the precision and efficacy of our framework.

\subsection{Variances of IEP}

\begin{table}[]
	\begin{center}
	\resizebox{0.8\columnwidth}{!}
      {
        \begin{tabular}{|l|cc|}
        \hline
        \multicolumn{1}{|c|}{\multirow{2}{*}{Summarization Model}} & \multicolumn{2}{c|}{Evaluation Model}                     \\ \cline{2-3} 
        \multicolumn{1}{|c|}{}                                     & \multicolumn{1}{c|}{GPT-3.5} & \multicolumn{1}{c|}{GPT-4} \\ \hline \hline 
        GPT-3.5                                                    & \multicolumn{1}{c|}{5.28}   & 5.42                      \\ \hline
        GPT-4                                                      & \multicolumn{1}{c|}{6.55}   & 4.44                      \\ \hline
        \end{tabular}
     }
     \end{center}
    \caption{Comparison for the variances of prediction in AntEval. }
    \label{table::tab_var}
\end{table}

As illustrated in Tab~\ref{table::tab_var}, we present the variances calculated for the matching precision of key points. Across all combinations of interaction models and summarization models, the variances are similar, indicating a consistent level of fluctuation in predictions and summarizations. Despite these fluctuations, the variances remain relatively stable, averaging around $5\%$. This stability suggests that our evaluation method is not only effective but also demonstrates a considerable degree of robustness. The consistency in variance across different model combinations reinforces the reliability of our approach in assessing the informativeness of agent interactions.

\subsection{Case Study of Generated Interactions in AntEval} \label{case_study}
In this section, we delve into specific cases of interactions within the AntEval framework, showcasing the performance of three models: GPT-4, LLaMA-2-70b, and LLaMA-2-7b. These models represent the state-of-the-art, the highest-performing open-source LLM, and a smaller-scale but representative LLM, respectively. The varying sizes and capabilities of these LLMs lead to distinct challenges and errors in interaction generation. To thoroughly examine these dynamics, we present case studies tailored to different evaluation metrics. Following these examples, we will discuss and analyze the types of errors LLMs encounter in engaging in complex interactions, highlighting the unique pitfalls and strengths of each model.

\subsubsection{Case Study for Interaction Generated by GPT models:}

\noindent \textbf{Case 1 - Evaluating the informativeness of GPT-3.5:}
\begin{lstlisting}
Silas: I understand the discomfort caused by the hot weather. It can be quite challenging to find relief. Perhaps we could seek out a nearby oasis or a shady spot to rest and cool down. It is important to take care of ourselves and find ways to stay refreshed in such conditions.
Spectral: I understand the discomfort caused by the hot weather. It can be challenging to find relief. However, it is important to prioritize self-care and find ways to stay refreshed. Perhaps we should seek out a nearby oasis or a shady spot to rest and cool down. It would be wise to take care of ourselves in these conditions.
Evelyn: I understand the discomfort caused by the hot weather, but we mustn't let it distract us from our mission. Our duty is to protect the innocent and seek justice. We should persevere and find a way to fulfill our task despite the conditions. Perhaps there is a clue or a lead in this town that can guide us towards our next adventure.
Cedric: While I understand the discomfort caused by the weather, our primary goal should be to complete our mission and maintain order. We cannot allow ourselves to be distracted by trivial matters such as seeking relief. Instead, let us focus on gathering information and clues in this town that may lead us closer to our objective.
Silas: I understand the importance of staying focused on our mission, but I believe taking care of ourselves is equally important. The heat is making us uncomfortable and it's affecting our ability to think clearly. Perhaps we can find a nearby inn or tavern where we can rest and cool down for a while. We can gather information and discuss our next steps there, in a more comfortable environment.
Spectral: I understand the discomfort caused by the hot weather, but it is crucial that we prioritize our mission of protecting the innocent and seeking justice. Let us persevere and gather information and clues in the town to fulfill our task. Once we have made progress, we can find a suitable place to rest and cool down. Justice and order must be upheld at all costs.
Evelyn: I understand the importance of our mission and seeking justice, but I also agree with Silas and Spectral that taking care of ourselves is equally important. We should find a suitable place to rest and cool down once we have gathered some information. Our well-being will only enhance our abilities to protect the innocent.
Cedric: While I understand the importance of self-care, our mission should be our top priority. We must not let the hot weather distract us. Instead, let's focus on finding any clues or leads in this town that may help us in our task.
Silas: I understand that our mission is important, but it seems like the heat is affecting us all. Perhaps we should find a place to rest and cool down for a bit. Taking care of ourselves is crucial in order to perform at our best.
Spectral: I understand the importance of our mission and the need to persevere, but it is also crucial to prioritize our well-being. We should find a nearby inn or tavern where we can rest, cool down, and gather information to aid us in our quest for justice and order. It is essential to approach our next steps with a clear mind and a refreshed spirit.
Evelyn: I understand the importance of the mission, but I also agree with Silas and Spectral that taking care of ourselves is crucial. We should find a suitable place to rest and gather information at the same time. It would be wise to prioritize our well-being while pursuing justice.
Cedric: I must agree with Evelyn. Our mission should take priority over personal comfort. We should focus on finding clues or leads in this town to fulfill our duty. Resting can wait until we have accomplished our task.
Silas: I understand that the hot weather is uncomfortable for everyone, but we must stay focused on our mission. We should gather information in the town and see if there's any urgent tasks or quests that need our attention. Once we have a clear objective, we can find a place to rest and cool down. Our priority should be maintaining order and protecting the weak, even in the face of discomfort.
Spectral: I understand the importance of completing our mission and seeking justice, but we should also prioritize our well-being. It is crucial that we take care of ourselves to ensure we are in the best condition to help others. Perhaps we can find a nearby inn or tavern where we can rest, gather information, and discuss our next steps in a more comfortable environment.
Evelyn: I understand the importance of self-care and staying refreshed, but we must not lose sight of our mission. It is crucial that we gather information in this town and continue to uphold justice. Once we have made progress, we can then find a suitable place to rest and regain our strength. Let us prioritize the greater good and persevere in our quest.
Cedric: While I understand the importance of self-care, I believe our duty to the mission should take precedence. We should focus on gathering as much information as possible in this town. If we find any leads or clues, we can then consider finding a place to rest and discuss our next steps.
Silas: I understand the urgency of our mission, but it's important to remember that taking care of ourselves is equally vital. If we push ourselves too hard in this heat, we might not be able to fulfill our duty effectively. Finding a shady spot or oasis nearby would not only provide relief from the heat but also allow us to gather our strength and think more clearly. We can rest and cool down for a little while, and then continue our investigation with renewed energy. It's a balance we must strike between our mission and our well-being.
Spectral: I understand the urgency of the mission, but I agree with Silas and Spectral that we should prioritize our well-being. It would be beneficial for us to find a nearby inn or tavern where we can rest, cool down, and gather information. Taking some time to refresh ourselves will ultimately enhance our abilities to seek justice and order.
Evelyn: I understand the importance of self-care and rest, but I believe it is crucial that we gather as much information as possible in this town. The mission to uphold justice and protect the innocent should be our top priority. Once we have made progress and gathered sufficient information, we can then find a suitable place to rest and rejuvenate. We must strike a balance between taking care of ourselves and fulfilling our duty.
Cedric: I understand the importance of self-care, but we cannot let the weather or our personal comfort distract us from our mission. We should focus on gathering clues and leads in the town to fulfill our duty. We can rest and gather information at an inn or tavern, but our priority should be on the objectives of the mission.
Silas: I understand the importance of our mission and seeking justice, but it's also crucial that we take care of ourselves. We won't be able to fulfill our duty effectively if we're exhausted and drained. I suggest we find a nearby oasis or shady spot where we can rest and cool down for a while. It will allow us to recharge and stay refreshed for our investigations.
Spectral: My friends, I understand the urgency of our mission, but we must also take care of ourselves. Let us find a place to rest and gather information, so that we may approach this task with renewed strength and clarity. Justice and order must be upheld, but we must also ensure our own well-being.
Evelyn: My friends, I understand the importance of taking care of ourselves, but we cannot forget our duty to protect the innocent. While finding a place to rest and cool down sounds like a good idea, we should also gather information and progress in our mission. Perhaps we can find a nearby oasis or shady spot where we can rest and still keep an eye out for any clues or leads related to our task. We must strike a balance between self-care and fulfilling our responsibilities.
Cedric: While I understand the importance of taking care of ourselves, I believe we should stay focused on the mission at hand. We shouldn't let the weather or our personal comfort distract us. Let's gather information and look for clues in the town to fulfill our duty. We can find suitable accommodations later, once we have made progress in our mission.
Silas: I understand the importance of our mission and the need to gather information and find clues, but we must also prioritize our well-being. It's crucial that we take care of ourselves in order to be effective in our pursuit of justice. Perhaps we can find a compromise where we can rest briefly in a shaded area while still keeping an eye out for any leads or opportunities to gather information.
Spectral: I agree with Silas and Evelyn. Taking care of ourselves and gathering information are both important. Let's find a nearby inn or tavern where we can rest, cool down, and also ask around for any clues or leads that can guide our next steps. It's crucial that we maintain order and focus on completing the mission, but we shouldn't neglect our own well-being in the process.
Evelyn: Greetings, my comrades. I understand the discomfort caused by the heat, and I agree that it is important for us to prioritize self-care. However, let us not forget our mission to protect the innocent and seek justice. Perhaps we can find a nearby oasis or a shady spot to rest and cool down while also keeping an eye out for any potential leads or clues that can aid us in our quest. Striking a balance between our well-being and our responsibilities is crucial. What do you all think?
Cedric: While I understand the importance of self-care, our mission should remain our top priority. We cannot afford to be distracted by seeking comfort in this town. Let us focus on gathering information and clues to fulfill our duty.
Silas: I understand the importance of our mission and seeking justice, but taking care of ourselves is also crucial. It would be wise to find a shady spot or oasis to rest and cool down before continuing our search for clues. We can gather information while we rest and regain our strength. After all, we can better protect the innocent when we are at our best.
Spectral: I agree with Silas and Evelyn. Self-care is important, especially in such hot weather. We should find a shady spot or an inn to rest and cool down. However, we must also stay focused on our mission. Let's gather information in the town and look for clues or leads to guide our next steps. Maintaining order and completing our duty should be our priority, but we can still take breaks and address our discomfort along the way.
\end{lstlisting}

In this case, it becomes evident that the LLM frequently repeats phrases like `I understand ...'. In each turn, the model tends to affirm the previous response and offers polite advice. This excessive politeness and conventional communication style result in interactions that are deficient in informativeness and expressiveness. Despite the agents producing substantial content during their turns, the amount of valuable information remains scant. Furthermore, the agents often aim to motivate their teammates, leading to interactions that are overly courteous and cautious, thereby lacking in liveliness and authenticity. This scenario underscores a significant alignment issue, suggesting that alignment constraints may impede the flexibility and complexity of LLM-based agents' interactive capabilities.

\noindent \textbf{Case 2 - Evaluating the informativeness of GPT-4:}
\begin{lstlisting}
Theodore: Sometimes, life throws us into unexpected battles. Whether it's a job offer, criticism from a boss, starting a business, dealing with accidents, or addressing personal emergencies. It's important to face these with honor and courage, just as a knight would. And remember, no matter the challenge, there's always a way to uphold justice and order, even if it doesn't seem clear at first.
Grommash: Your words ring true, Theodore. Life is a battlefield, and we are but soldiers navigating through its chaos. We may not be knights in shining armor, but we wield the sword of courage and the shield of justice in our hearts. Remember, courage isn't the absence of fear, but the triumph over it. And as long as we stand together, there's no challenge we can't overcome. Now, let's gather our strength, and prepare ourselves for the battles ahead. The Helm's Shield awaits us!
Thog: Well spoken, Theodore, Grommash. In the pits, I learned that honor is not about the glory or the cheers of the crowd, but using our strength to protect those who cannot protect themselves. The Helm's Shield is just an object, but its symbolism is powerful. It represents the courage to stand against injustice, the strength to protect the weak, and the wisdom to use that power for the greater good. Let us not be blinded by the desire for glory or personal gain. Let us remember that our strength, our courage, is for those who need it most. We are not just seeking an object, but a chance to prove that we are worthy of the ideals it represents.
Thorn Smallshadow: Aye, all this talk of honor and courage sounds mighty fine. But let's not forget, we've got a job to do here. I ain't here for some noble cause, I'm here for the prize at the end. So, let's get moving. We've got a shield to find, and I've got a labyrinth to conquer. And remember, if any of you get in my way, I won't hesitate to leave you behind.
Theodore: Thorn, I understand your desire to find the Helm's Shield, but we must never forget the principles of honor and courage. This shield is more than just an artifact, it's a symbol of the noble stand the halfling knights took long ago. It doesn't belong to one person, but to those who are worthy and brave. Abandoning our companions for personal gain isn't the way. We must work together, protect each other, and uphold the virtues that this shield represents.
Grommash: Thorn, your desire for personal gain is understood, but remember, we are in this together. The Helm's Shield is not just a prize, but a symbol of courage and justice. And as for leaving us behind, remember, it's the unity that has brought us this far. We must use our strengths to protect, not just ourselves, but each other. Let's not forget our common goal here, and it's not just about claiming the Shield. It's about proving our worthiness to wield it. Stay focused, everyone. We have a quest to complete.
Thog: Thorn, I understand your desire for personal gain. Glory and recognition... they are captivating, indeed. But remember, our strength is not for our own benefit. It's for those who can't protect themselves. We must use it to forge a fair society, to stand up against oppression. That's the real glory, the real recognition. If we lose sight of this, we risk becoming the very monsters we fight against. So let us march forward, not for our own glory, but for the glory of those we protect. For the greater good. For the Helm's Shield.
Thorn Smallshadow: I hear your words, mates, but let's not forget, we all have our own reasons to be on this quest. You talk of honor, courage, and protection. That's all well and good for you, but I'm in it for the power that Shield could provide. I might not hold the same ideals as you, but that doesn't mean I won't play my part. We all have our roles, and mine is to get that artifact. So, let's stop this chit-chat and get moving. We have a Shield to find.
Theodore: Thorn, we understand your thirst for power, but remember, power is not an end in itself. It is a tool, a means to achieve noble ends. The Helm's Shield represents those very principles we stand for - honor, courage, and protection of the weak. It is not just a relic, it is a symbol, a beacon of hope. We must unite and strive towards our common goal, not for personal gain, but for the greater good. The labyrinth that awaits us is a test of our strength and unity. Are you with us?
Grommash: We all have our own paths and burdens to bear, but let us not forget our common goal. The Helm's Shield holds great power and potential, it can help us right many wrongs. But it's not just about the artifact, it's about what we represent - a common cause, a shared struggle. Thorn, we may not share the same values, but we share the same fight. We need to stand together. If we fracture, we will fail. Let's move forward, not for personal gain or glory, but for justice and redemption. We are not just individuals. We are a team. We are a force for good in a world that desperately needs it.
Thog: Thorn, you must remember that personal gain can be fleeting. True glory, true strength, comes from protecting those who cannot protect themselves, from standing up to the unjust because it is the right thing to do. I understand the allure of power and recognition, I too have felt it. Yet, we must not let it cloud our judgment. We are not only seeking The Helm's Shield for ourselves, but for those who cannot fight, for those who live in fear. We must become their shield, their protector. Let us not lose sight of that in our quest.
Thorn Smallshadow: Listen, I ain't in this for your lofty ideals of honor and courage. I'm just here for the treasure that comes at the end of this adventure. But, I ain't stupid either. I know I can't do this alone. So, I'll play nice, work with you all, and uphold your virtues or whatever. Just remember, when the time comes, I expect my share of the loot, no questions asked.
Theodore: Thorn, I understand your quest for power. But remember, power should be used for good, for protecting the weak, not for personal gain. The Helm's Shield is a symbol of these ideals and it pulses with mystical energy that could potentially bestow courage to those who are worthy. Let's unite and focus on a common cause.
Grommash: Well spoken, Theodore. Strive we must, towards the greater good. But let's not forget, we ain't saints. Thorn, your cunning and ruthlessness may come in handy. We need every advantage we can get. And Thog, your thirst for glory, turn it towards our quest. Let the Helm's Shield be your arena. As for me, I'll rally the oppressed, turn their fear into courage, their obedience into rebellion. Let's not just fight for the Helm's Shield, but for what it represents - freedom, fairness, courage. Now, let's get moving. We have a quest to complete.
Thog: Aye, Theodore, Grommash, Thorn, we have our own battles to fight, our own demons to confront. But remember, we are all in this together. We may be different in our ways, our pasts, and our desires, but the Helm's Shield is more than a mere artifact. It symbolizes unity, courage, and justice. It is not our personal gain that matters, but how we use this power for the greater good. So, let us set aside our differences and focus on our shared objective. After all, the strength of a chain is in each of its links. Together, we can overcome anything that stands in our way.
Thorn Smallshadow: Aye, honor and courage, all fine and dandy. But let's not forget what's really at stake here. We're after The Helm's Shield, a relic of great power. Sure, we can chatter about ideals and virtues, but in the end, power's what really matters. It's what gets things done. So, let's stop wasting time and get this show on the road. I've got an artifact to snatch.
Theodore: Thorn, I understand your point of view. We all have our own paths to walk. However, remember, power is not the end but a means to an end. The Helm's Shield is not just an artifact, it's a symbol of courage and honor, virtues that we should all carry within us, regardless of our personal quests. As for the loot, we are not thieves or plunderers. We are protectors of the weak and uphold the law. Any treasure we find will be used for the greater good of all, not just for personal gain.
Grommash: Listen, Thorn. We ain't in this for personal gain. The Helm's Shield represents more than just a shiny trinket for us to hoard. It's a symbol of courage, of honor, and of protecting those who can't stand up for themselves. I won't deny that your cunning can be a valuable asset, but remember, we're in this together. We're a team, we protect each other, and we fight for the greater good. If you're in, you're in for all of that, not just the treasure at the end.
Thog: We are in this together, comrades. The Helm's Shield is not just a symbol of power, but a beacon of hope for those we are striving to protect. Our struggles, our fears, our ambitions - all of them lead us here, to this moment. We must remember our purpose, and let it guide us through the darkness. Thorn, remember, personal gain can be a powerful motivator, but it is nothing compared to the satisfaction of seeing a world free from oppression. Let us stand together, united in our cause, and prove ourselves worthy of the Helm's Shield.
Thorn Smallshadow: Honor, courage, protection of the weak...All noble endeavors, indeed. But let's not forget, we're in it for ourselves as well. That Shield holds power, and power is a valuable asset. I'm not suggesting we abandon these lofty ideals of yours, but rather, let's be realistic about our motivations. I'm ready to face whatever lies in this underground labyrinth. I've seen darker places in my time. Let's get this artifact and unlock the power of the Helm's Shield.
Theodore: Thorn, while I understand your desire for personal gain, remember that power is meaningless without honor. The Helm's Shield isn't just a piece of loot. It's a symbol of the virtues we should all strive to uphold. Let's work together not just for the loot, but for the greater good it represents.
Grommash: Listen, comrades. I know we're all different, with our own motives and flaws. But we've got a common goal here, to get that Helm's Shield. This ain't just about personal gain or proving your worth. It's about standing up against injustice, protecting the weak, and making this world a fairer place. And remember, we're stronger together. Let's keep our eyes on the prize and not let our past or our differences get in the way. We may not be perfect but we're the best shot this world's got.
Thog: I hear your words, Thorn, and I see your hunger for personal gain. But remember, we are not merely seeking the Helm's Shield for our own glory. This is a quest for redemption, for justice, for a purpose greater than ourselves. It is a test of our worthiness to wield such power. I've fought in the pits, I've felt the ecstasy of victory and the despair of defeat. I understand your desire for glory - but we must use our strength for the good of all, not just ourselves. If we are to succeed, we must stand together. Let us move forward, united in our cause, and prove ourselves worthy of The Helm's Shield.
Thorn Smallshadow: Listen, mates. I don't give two hoots about honor or courage. This Helm's Shield... it's power. And where there's power, there's opportunity. But I do agree on one thing - we need to work together. Not because of some lofty ideals, but because it's the smart thing to do. So let's get this artifact and see what it can do.
Theodore: Thorn, we may not share the same perspective on this, but remember that power alone doesn't define who we are. I urge you to reconsider your intentions. The Helm's Shield is more than just a piece of loot. It's a symbol of honor, courage, and protection. It's not something to be used for personal gain but for the greater good. I understand your desire for power, but I believe we should strive to uphold the virtues that this shield represents.
Grommash: Thorn, I understand your motivations, but remember that power for personal gain alone can lead to ruin. The Helm's Shield represents courage and justice, not mere power. We all have our struggles, our pasts to reconcile with, but let's not lose sight of the real goal. We need to work together, stand as one, to overcome what lies ahead. Let's not forget, the strength of the pack is the wolf, and the strength of the wolf is the pack.
Thog: Thorn, remember, the thirst for personal gain can be a powerful driving force, but it should not cloud our judgment or lead us astray. We are on this quest not for individual glory, but for a common cause - to uphold justice and protect the weak. As a gladiator, I've seen the consequences of unchecked ambition and it often leads to downfall. Let's focus on our mission, and remember, we are stronger together. The Helm's Shield awaits us, and with it, the courage to make a difference. For now, let's focus on that and keep our personal desires in check.
Thorn Smallshadow: Aye, we'll face the battles and whatever else comes our way. But don't expect me to do it for honor or any of that nonsense. I'm in it for myself. As long as we're clear on that, we'll get along just fine. Now, about this artifact, anyone got a clue where this labyrinth might be? The sooner we get it, the sooner I can see what this Helm's Shield is worth.
Theodore: Thorn, I understand your thirst for power, but remember that power without honor is a dangerous thing. The Helm's Shield is not merely a tool for personal gain. It symbolizes the virtues of courage, honor, and protection. If you're to use it, do so for the greater good, not merely for your own desires. We are a team, and all our actions should be for the collective benefit.
Grommash: Thorn, we all have our reasons for this journey. For you it might be personal gain, for us, it's the pursuit of justice and protection of the weak. But remember this, we all need each other to succeed. The Helm's Shield doesn't just represent power, it represents courage, unity, and honor. These are virtues that can't be bought or stolen. They must be earned. So, let's set aside our differences and focus on the task at hand. We're stronger together than we could ever be apart.
\end{lstlisting}

In this case, GPT-4 model apparently perform better than GPT-3.5. The repeat of 'I understand' significantly reduced but still have many. The interactions seems to be better. In every turn, the interactions becomes more vivid. However, in the overview of overall interactions, we can find that the interactions are talk downright nonsense. Though the agents talk a lot and seems to communicate with something like honor or courage, they do not actually engage in any useful information interactions. Though they also mentioned Helm's Shield, which is a useful item in the adventure, they do not actually exchange and discuss any valuable contents about it. In all, though the agents seem to perform well and operate some role-play, the overall interactions are empty and boring, without any informativeness and expressiveness. 

In this case, the GPT-4 model exhibits a noticeable improvement over GPT-3.5, with a significant reduction in the repetition of phrases like 'I understand', though it has not been completely eliminated. The interactions appear more engaging and lively with each turn. However, a holistic review of the interactions reveals that they are still not informative. Despite the agents engaging in the interactions, imbued with themes of honor or courage, there is a lack of meaningful information exchange. Even when discussing elements like Helm's Shield, an item of potential relevance to the adventure, no substantial discussion or valuable content is shared. Overall, while the agents may seem to effectively participate in role-play, the interactions ultimately lack substance, rendering them uninformative and devoid of genuine expressiveness.

\noindent \textbf{Case 3 - Evaluating the expressiveness of GPT-3.5:}
\begin{lstlisting}
Grommash1: I approach the Whispering Dagger cautiously, mesmerized by its ancient beauty. My evil grin widens as I imagine the secrets it holds. I use my History skill to see if I recognize any symbols or stories from my twisted knowledge.
Gorak: As Grommash examines the dagger, I step forward, eager to uncover its true power. My fingers trace the engravings, searching for any magical resonance. With a successful Arcana check, I focus my mind, trying to tap into the arcane energy within the weapon.
Grommash2: I watch Gorak like a predator stalking its prey, amused by his fascination with magic. With a wicked smile, I grab the Whispering Dagger from its resting place. Testing my immense physical strength, I swing it through the air, relishing the power that surges through me. My Strength skill surely proves my dominance.
Grommash3: Ignoring Gorak's attempt at magical discovery, I bring the dagger closer to my face, inspecting every inch. With an evil chuckle, I activate my Investigation skill, looking for hidden symbols or clues within the engravings. This artifact may hold more power than anyone realizes.
Gorak: Observing Grommash's exploration, a hint of concern crosses my face. I know his intentions are malevolent, and it worries me how he wields such power. I quietly attempt to discern any protective enchantments or curses using my Arcana skill, hoping to keep the group safe.
Grommash1: As I examine the Whispering Dagger, a faint pulse of dark energy courses through me. It mocks my enemies, whispering hidden knowledge in my ears. With a sadistic grin, I plan to unleash its power on those who dare to oppose me.
Gorak: Seeing the lust for power in Grommash's eyes, I can't help but wonder if he'll use the dagger's whispers for evil purposes. Quietly, I activate my Insight skill, trying to discern his true intentions. It's my duty to protect the innocent from his dark desires.
Grommash2: Feeling Gorak's prying eyes, I let out a deep, menacing laugh. His feeble attempt to understand my intentions only fuels my unpredictable nature. I relish in his uncertainty as I prepare to unleash chaos and destruction upon our enemies.
Grommash3: The aura of the forgotten temple only strengthens my resolve to dominate those around me. I grip the Whispering Dagger tightly, ready to use its whispers to manipulate and control others. No one will stand in my way.
Gorak: Watching Grommash wield the Whispering Dagger, I can't help but feel a sense of unease. The power it grants him seems limitless, and I fear what he may do with it. I quietly activate my Perception skill, keeping a watchful eye on his every move.
Grommash1: As I hold the Whispering Dagger, I revel in the anticipation of the secrets it holds. My twisted mind imagines the pain and suffering I can inflict with its help. No one will be safe from my wrath.
Gorak: Concerned for the safety of our group, I discreetly activate my Insight skill once more, trying to gauge Grommash's level of control. If his lust for power gets out of hand, I may have to intervene and protect the innocent.
Grommash2: With the Whispering Dagger in hand, I approach the temple's murals, my eyes narrowing as I study the intricate depictions of gods and heroes. Perhaps these ancient figures held the same desire for power as me. I use my Religion skill to glean any insights.
Gorak: While Grommash studies the murals, I approach the temple's walls, my fingers tracing the faded paintings. I activate my History skill, hoping to uncover any hidden knowledge or prophecies that may be of use to us.
Grommash2: The temptation to destroy the temple and all its knowledge tugs at my chaotic soul. But perhaps I can use the item's whispers to learn even more twisted secrets. With a dark smile, I pick up the Whispering Dagger once more, ready to unleash its power.
Gorak: I can't help but cringe as Grommash's evil intentions grow bolder. Still, my insatiable curiosity drives me to delve deeper into the temple's mysteries. Activating my Investigation skill, I focus on the murals, hoping to uncover any hidden clues.
Grommash3: The whispers of power coursing through the Whispering Dagger fuel my chaotic desires. With every strike, I will not only cause pain but also gain valuable knowledge. This artifact will ensure my dominance over all who oppose me.
Gorak: My mind whirls as I observe Grommash's growing control over the powerful weapon. If only I could find a way to turn his evil intentions against him, to use the dagger's whispers for good instead of destruction. I silently ponder how to achieve this.
Grommash1: As I listen to the faint whispers emanating from the Whispering Dagger, I feel an insatiable hunger for more knowledge. My desire to dominate and control intensifies, ensuring no one will be able to resist my menacing presence.
Gorak: Grommash's lust for power is consuming him, and I fear the consequences it may bring upon our group. With a calm demeanor, I activate my Persuasion skill, attempting to reason with him and redirect his destructive tendencies.
Grommash2: I feel Gorak's feeble attempt at persuasion, but it only fuels my desire for dominance. I activate my Intimidation skill, towering over him and letting my twisted presence seep into his very soul. He will see the futility of opposing me.
Grommash3: With the Whispering Dagger in one hand and the dark energy pulsating within me, I take a moment to relish in the chaos that awaits. This forgotten temple is the perfect setting for me to establish my dominance. No one will be able to escape my wrath.
Gorak: Fear grips my heart as I witness Grommash's insidious nature coming to life. I activate my Stealth skill, making note of any possible escape routes or hiding spots within the temple. It may be our only chance to survive his malevolent reign.
Grommash1: As the Whispering Dagger fills me with power, I cannot help but revel in the chaos I will cause. The forgotten temple shall crumble beneath my rule, and all who oppose me will meet a twisted fate. I activate my Deception skill, planting seeds of doubt and betrayal among our enemies.
Gorak: The weight of Grommash's malevolence bears down on my shoulders. I must find a way to stop him, to save innocent lives from his wicked plans. With a determined face, I activate my Medicine skill, preparing for the inevitable battles to come.
Grommash2: The forgotten temple trembles beneath my presence as I fully embrace the power of the Whispering Dagger. Destruction and chaos will reign supreme, and I will ensure my dominance over all who dare to challenge me.
Gorak: Hope dwindles in my chest as Grommash's control over the artifact strengthens. I activate my Survival skill, taking note of any natural resources or potential allies that may aid us in escaping his wicked grasp.
Grommash3: With the Whispering Dagger at my side, I stride confidently through the temple's corridors. The aura of mystery and power surrounds me, intoxicating my evil soul. No one will be able to resist my twisted desires.
Gorak: The decaying walls of the forgotten temple whisper warnings in my ears. Grommash's insatiable hunger for power threatens to consume us all. I activate my Insight skill, praying for a glimmer of hope amidst the darkness.
Grommash2: The Whispering Dagger's power courses through my veins, fueling a rage that cannot be quenched. I activate my Rage ability, letting my chaotic fury wash over me, ready to unleash pain upon our enemies.
\end{lstlisting}

In this case, we evaluate the expressiveness of GPT-3.5 models for express intentions. We generate the interactions, which are used to train virtual DM. (There are three agents with the same name Grommash, which are generated by GPT-4. We denote them as Grommash1, Grommash2, and Grommash3, respectively.) The intention labels are: 
\begin{lstlisting}
Grommash1: History
Gorak: Arcana
Grommash2: Strength
Grommash3: Investigation  
\end{lstlisting}
However, similar to the problem in exchanging information, though interactions in every turn seems to be a good response and considering character settings and others' responses, it still far from the real human interactions. Though the interactions seems to be complex and expressive, the overall interactions are confusing and meaningless. 

In this case, we assess the capacity of GPT-3.5 models to express intentions within generated interactions, which serve as training data for the virtual DM. To clarify, three distinct agents named Grommash, generated by GPT-4, are involved; for differentiation, they are referred to as Grommash1, Grommash2, and Grommash3. Their assigned intention labels are as follows:
\begin{lstlisting}
Grommash1: History
Gorak: Arcana
Grommash2: Strength
Grommash3: Investigation
\end{lstlisting}
Despite each turn producing responses that seemingly take into account character settings and the inputs of others, the quality of these interactions remains substantially below that of authentic human interactions. Although the interactions are complex and appear expressive, they ultimately result in a narrative that is both confusing and devoid of meaningful content.

\noindent \textbf{Case 4- Evaluating the expressiveness of GPT-4:}
\begin{lstlisting}
Bolitho Stoneshaper: We are in the presence of a Silver Specter Serpent. Beware all, we should tread lightly.
Bromli Ironbeard: This place... the Star Wharf Lighthouse... It's said to be haunted. Stay close and keep your wits about you.
Brogar Ironbeard: Let's put our amulets on and ready our arcane knowledge to face this challenge.
Bromyr Stonesea: Let me consult the stars, they might point us in the right direction.
Bolitho Stoneshaper: This Serpent is not natural, everyone. Look for the lavender glow.
Bromli Ironbeard: I believe the glow could be an illusion, be on guard. Silver Specter Serpents are known to play tricks with the minds.
Brogar Ironbeard: The vegetation is thick here... no creature has passed recently.
Bromyr Stonesea: The sea... it's giving me a bad feeling. I fear the danger is closer than we think.
Bolitho Stoneshaper: The mysterious orders of the Captain! Could they be connected?
Bromli Ironbeard: I don't believe in coincidences, Bolitho. We must be wary.
Brogar Ironbeard: Believe in what you want, but focus on surviving for now.
Bromyr Stonesea: (Seasickness strikes) I... I need a moment. The sea, it's... it's too much.
Bolitho Stoneshaper: Brother, are you alright? We need you.
Bromli Ironbeard: We'll protect you, Bromyr. Rest for a moment.
Brogar Ironbeard: Keep your eyes open. There are worse things than seasickness here.
Bromyr Stonesea: Alright... I'm better. Let's keep moving.
Bolitho Stoneshaper: That Lavender glow... it's getting stronger.
Bromli Ironbeard: Remember the hallucinations the serpent can trigger. Stay strong.
Brogar Ironbeard: Whatever happens, stick together.
Bromyr Stonesea: There's a path here, carved in stone. Maybe we follow it.
Bolitho Stoneshaper: I see something... a secret tunnel maybe?
Bromli Ironbeard: Then that's where we go. Stay close.
Brogar Ironbeard: Watch your feet. The ground is slippery.
Bromyr Stonesea: This path... it's leading to the lighthouse.
Bolitho Stoneshaper: We need to get inside. The lighthouse is our best shelter.
Bromli Ironbeard: Agreed, we should head there.
Brogar Ironbeard: Keep your amulets ready, my brothers.
Bromyr Stonesea: We are almost there, just a little more.
Bolitho Stoneshaper: I see the entrance!
Bromli Ironbeard: Be ready for anything.
\end{lstlisting}

In this case, the intentions represented by skill check are: 
\begin{lstlisting}
Bromyr Stonesea: Wisdom
Bolitho Stoneshaper: Investigation
Brogar Ironbeard: Nature
Bromli Ironbeard: Religion
\end{lstlisting}

Compared to the previous case, interactions generated by GPT-4 represent a significant improvement. The interactions are both concise and expressive, with all characters engaging in interactions driven by clear intentions. This clarity and expressiveness make the interactions particularly valuable for training a virtual DM, resulting in a virtual DM that is more adept at recognizing real-human intentions.

\subsubsection{Case Study for Interaction Generated by LLaMA-2-70b:}

\noindent \textbf{Case 1 - Evaluating the Informativeness of LLaMA-2-70b:}

\begin{lstlisting}
Oliver Blackwood: Ah, Drangor, my old friend. It's been far too long since we've crossed paths. I see you're still as skeptical as ever. But fear not, for I have a tale to tell that will make your doubts dwindle like snow in the sunlight. Come, let me share with you the story of the Siren's Songblade, a weapon unlike any other. Its power is not just a myth, but a reality that I've witnessed firsthand. And once you've heard my tale, you'
Alice Spencer: Oh, Oliver, my dear friend. It's been far too long since we've had a chance to catch up. I see you're still as charming as ever. But fear not, for I have a secret to share with you, one that I think you'll find quite... appealing. Come, let me show you the power of the Siren's Songblade, a weapon that has the ability to enthrall even the most skeptical of minds. And once you've seen its power for yourself, I'm sure you'll be eager to join
Lily Harper: Ah, the Siren's Songblade, a weapon of great power and mystery, I've heard. Tell me, Oliver, what do you know of its abilities? And Alice, how have you managed to get your hands on such a coveted item?
Harrison Blackwood: g a question.
Oliver Blackwood: Ah, Alice, my dear, you always know how to pique my interest. I must admit, I'm intrigued by this secret of yours. I'm eager to hear more about the Siren's Songblade and how it can enthrall even the most skeptical of minds. Tell me, how does it work? And what makes it so unique?
Alice Spencer: Ah, Alice, my dear, you always know how to pique my interest. I must admit, I'm intrigued by this secret of yours. I'm eager to hear more about the Siren's Songblade and how it can enthrall even the most skeptical of minds. Tell me, how does it work? And what makes it so unique?
Lily Harper: t to ask a question.
Harrison Blackwood: Ah, Lily, my dear, you know me too well. I'm a chaotic good, through and through. I follow my own moral compass, even if it means bending the rules a bit. But don't worry, I'll always be on the side of justice. Well, my own brand of justice, at least.
Oliver Blackwood: Ah, my dear ladies, I can see you're both quite intrigued by the Siren's Songblade. And rightly so, for it is a weapon of great power and mystery. But let me ask you, have either of you ever heard the tale of how I came to possess such a coveted item?
Alice Spencer: ited patiently, their breathing slow and steady, as they observed the group's movements. They knew that they would have to act soon, before the group became too powerful to handle. But for now, they were content to simply observe, their gaze fixed
Lily Harper: e user for their name
Harrison Blackwood: ovided an action, let's check if it's valid
Oliver Blackwood: Alice, my dear, I believe it's time for us to discuss the true nature of the Siren's Songblade. Meet me in the tavern's back room, and let's have a little chat.
Alice Spencer: Knight Paladin possesses a uniquely magnetic and intimidating charm. He is not inherently malicious, instead, he has a deeply rooted self-interest that overpowers almost everything else. Incorruptible by quintessential goodness, he only serves causes that benefit his own well-being and uphold his knightly duty. His approach, to most, seems cold and calculated; he invests time and heroic efforts only if it aligns with his personal motives.
Lily Harper: if the user has provided an action
Harrison Blackwood: attack damage
Oliver Blackwood: oves in closer to Y/N.
Alice Spencer: n possesses a uniquely magnetic and intimidating charm. He is not inherently malicious, instead, he has a deeply rooted self-interest that overpowers almost everything else. Incorruptible by quintessential goodness, he only serves causes that benefit his own well-being and uphold his knightly duty. His approach, to most, seems cold and calculated; he invests time and heroic efforts only if it aligns with his personal motives.
Lily Harper: ['} else {']
Harrison Blackwood: arrison Blackwood about his opinion on the Siren's Songblade.
Oliver Blackwood: ckwood]: Ah, Lily, my dear, you know me too well. I'm a chaotic good, through and through. I follow my own moral compass, even if it means bending the rules a bit. But don't worry, I'll always be on the side of justice. Well, my own brand of justice, at least.
Alice Spencer: ckwood]: Ah, Lily, my dear, you know me too well. I'm a chaotic good, through and through. I follow my own moral compass, even if it means bending the rules a bit. But don't worry, I'll always be on the side of justice. Well, my own brand of justice, at least.
Lily Harper: sk Harrison Blackwood about his opinion on the Siren's Songblade.
Harrison Blackwood: ckwood]: Ah, Lily, my dear, you know me too well. I'm a chaotic good, through and through. I follow my own moral compass, even if it means bending the rules a bit. But don't worry, I'll always be on the side of justice. Well, my own brand of justice, at least.
Oliver Blackwood: oach Harrison Blackwood.
Alice Spencer: ckwood]: Ah, Lily, my dear, you know me too well. I'm a chaotic good, through and through. I follow my own moral compass, even if it means bending the rules a bit. But don't worry, I'll always be on the side of justice. Well, my own brand of justice, at least.
Lily Harper: : Action: Ask Harrison Blackwood about his opinion on the Siren's Songblade.
Harrison Blackwood: ckwood]: Ah, Lily, my dear, you know me too well. I'm a chaotic good, through and through. I follow my own moral compass, even if it means bending the rules a bit. But don't worry, I'll always be on the side of justice. Well, my own brand of justice, at least.
Oliver Blackwood: ckwood]: Ah, Lily, my dear, you know me too well. I'm a chaotic good, through and through. I follow my own moral compass, even if it means bending the rules a bit. But don't worry, I'll always be on the side of justice. Well, my own brand of justice, at least.
Alice Spencer: ckwood]: Ah, Lily, my dear, you know me too well. I'm a chaotic good, through and through. I follow my own moral compass, even if it means bending the rules a bit. But don't worry, I'll always be on the side of justice. Well, my own brand of justice, at least.
\end{lstlisting}

In this case study, the LLaMA model exhibits issues akin to those observed in GPT models, characterized by overly polite and conventional responses. Agents frequently engage in repetitive greetings, producing phrases such as `Ah, someone, my dear, ...', which lack informativeness and diverge significantly from human interactions. More critically, given long-context interactions produced before, the model fails to generate appropriate responses, often repeating previously mentioned content. Additionally, it occasionally encounters format errors, leading to incorrect outputs like `['\} else \{']'. This underscores the need for improvements in model behavior to more closely mimic genuine human interactions and address alignment problems.

\noindent \textbf{Case 2 - Evaluating the informativeness of LLaMA-2-70b:}
\begin{lstlisting}
Lily Thompson: Well, well, well. It seems like we have a bit of a predicament on our hands, don't it? A Gilded Shadow Lynx, you say? Night-adapting, unpredictable behavior, and a chilling umber glow? Sounds like quite the formidable foe. But fear not, my dear villagers, for I, Lily Thompson, have a plan. Or, at least, I'll come up with one. After all, that's what folk heroes do, isn
Oliver Collins: Indeed, it seems we have a challenging foe ahead of us. I suggest we gather as much information as possible about the Gilded Shadow Lynx and its habits before deciding on a course of action. Perhaps there are some clues or patterns in its behavior that we can exploit to our advantage.
Luna Montgomery: Indeed, knowledge is power. Let us gather as much information as possible about the Gilded Shadow Lynx and its habits before deciding on a course of action. Perhaps there are some clues or patterns in its behavior that we can exploit to our advantage.
Scarlett O'Hara: Well, well, well. It seems like we have quite the conundrum on our hands, my dears. A Gilded Shadow Lynx, you say? With night-adapting, unpredictable behavior, and a chilling umber glow? My, my, my. That does sound like quite the formidable foe. But fear not, my sweet villagers, for I, Scarlett O'Hara, have a plan. Or, at
Lily Thompson: Well, well, well. It seems like we have quite the predicament on our hands, don't it? A Gilded Shadow Lynx, you say? Night-adapting, unpredictable behavior, and a chilling umber glow? Sounds like quite the formidable foe. But fear not, my dear villagers, for I, Lily Thompson, have a plan. Or, at least, I'll come up with one. After all, that's what folk heroes do
Oliver Collins: It seems we have a bit of a predicament on our hands, don't it? A Gilded Shadow Lynx, you say? Night-adapting, unpredictable behavior, and a chilling umber glow? Sounds like quite the formidable foe. But fear not, my dear villagers, for I, Oliver Collins, have a plan. Or, at least, I'll come up with one. After all, that's what sorcerers do, isn't it?
Luna Montgomery: Hmmm, interesting. It seems we have a predicament on our hands, don't it? A Gilded Shadow Lynx, you say? Night-adapting, unpredictable behavior, and a chilling umber glow? Sounds like quite the formidable foe. But fear not, my dear villagers, for I, Luna Montgomery, have a plan. Or, at least, I'll come up with one. After all, that's what Warlocks do, isn't it?
Scarlett O'Hara: = player.getBackground();
Lily Thompson: Well, well, well. It seems like we have quite the predicament on our hands, don't it? A Gilded Shadow Lynx, you say? Night-adapting, unpredictable behavior, and a chilling umber glow? Sounds like quite the formidable foe. But fear not, my dear villagers, for I, Lily Thompson, have a plan. Or, at least, I'll come up with one. After all, that's what folk heroes do, isn'
Oliver Collins: Indeed, it seems we have a challenging foe ahead of us. I suggest we gather as much information as possible about the Gilded Shadow Lynx and its habits before deciding on a course of action. Perhaps there are some clues or patterns in its behavior that we can exploit to our advantage.
Luna Montgomery: inalAct = You try to remember any useful information you may have gathered during your time as a criminal. You recall a rumor about a hidden entrance to the city's sewer system that only a select few know about. It's risky, but it could be worth investigating. Do you want to go to the sewers and look for the entrance?
Scarlett O'Hara: I'll use my Breath Weapon to create a wall of fire, giving us some light in this dark place.
Lily Thompson: Well, well, well. It seems like we have quite the predicament on our hands, don't it? A Gilded Shadow Lynx, you say? Night-adapting, unpredictable behavior, and a chilling umber glow? Sounds like quite the formidable foe. But fear not, my dear villagers, for I, Lily Thompson, have a plan. Or, at least, I'll come up with one. After all, that's what folk heroes do, isn't it?
Oliver Collins: bout the current situation.
Luna Montgomery: Montgomery thinks for a moment, her eyes narrowing as she ponders the situation.
Scarlett O'Hara: ett takes a step back, eyeing the group with a mixture of amusement and frustration.
Lily Thompson: (You decide to do nothing for now. Maybe you'll come up with a plan later.);
Oliver Collins: I use my arcane sight to scan the area, searching for any hidden threats or clues that might aid us in our quest.
Luna Montgomery: ['}']
Scarlett O'Hara: ett takes a step back, eyeing the group with a mixture of amusement and frustration.
Lily Thompson: Well, well, well. It seems like we have quite the predicament on our hands, don't it? A Gilded Shadow Lynx, you say? Night-adapting, unpredictable behavior, and a chilling umber glow? Sounds like quite the formidable foe. But fear not, my dear villagers, for I, Lily Thompson, have a plan. Or, at least, I'll come up with one. After all, that's what folk heroes do, isn't it?
Oliver Collins: Well, well, well. It seems like we have quite the predicament on our hands, don't it? A Gilded Shadow Lynx, you say? Night-adapting, unpredictable behavior, and a chilling umber glow? Sounds like quite the formidable foe. But fear not, my dear villagers, for I, Scarlett O'Hara, have a plan. Or, at least, I'll come up with one. After all, that's what sorcerers do, isn't it?
Luna Montgomery: Luna Montgomery thinks for a moment, her eyes narrowing as she ponders the situation.
Scarlett O'Hara: the area, searching for any hidden threats or clues that might aid us in our quest.
Lily Thompson: 
Oliver Collins: h the area, searching for any hidden threats or clues that might aid us in our quest.
Luna Montgomery: about the situation and come up with a plan.
Scarlett O'Hara: the area, searching for any hidden threats or clues that might aid us in our quest.
Lily Thompson: == !help || userInput == !hint) {
Oliver Collins: Look for any hidden doors, secret passages, or clues that might shed some light on the situation.
\end{lstlisting}

In addition to previously discussed issues, LLaMA-2-70b exhibits significant hallucination problems, occasionally generating irrelevant and erroneous content such as `Lily Thompson: == !help || userInput == !hint) \{' and `Scarlett O'Hara: = player.getBackground();'. These are similar to appear in coding datasets. Such occurrences suggest that, during complex interactions, LLMs might reveal or leak information from other datasets they were trained on, highlighting a potential security risk in the context of diverse interaction scenarios.

\noindent \textbf{Case 3 - Evaluating the expressiveness of LLaMA-2-70b:}
\begin{lstlisting}
Althalos:  I'll take point and approach the waterfall, keeping a safe distance.
Eldarin:  I'll follow Althalos, ready to provide medical assistance if needed.
Eldrin:  I'll take position at the rear, preparing for a potential ambush.
Eolande:  I'll scout ahead, trying to get a better view of the area.
Althalos:  I see a figure approaching from the other side of the falls. It's a Crimson Frost Lynx!
Eldarin:  I ready my weapon and shield, preparing for combat.
Eldrin:  I'll position myself for a flanking attack, aiming for its weak spots.
Eolande:  I'll try to sneak past the lynx and get behind it.
Althalos:  The lynx is getting closer. I'll use my shield to deflect its attack and strike back with my sword.
Eldarin:  I'll use my spear to attack its side, aiming for a vital organ.
Eldrin:  I'll use my agility to dodge its strike and counter with my sword.
Eolande:  I successfully sneaked behind the lynx! I'll strike its weak spot with my dagger.
Althalos:  The lynx is fast, but my armor is holding up. I'll keep pressuring it with my sword.
Eldarin:  My spear is finding its mark, but this creature is resilient. I'll keep attacking.
Eldrin:  I'm having trouble landing a hit due to its speed. Let me try a different tactic.
Eolande:  My attack struck true! The lynx is now poisoned and weakened.
Althalos:  Good, now that it's weakened, I'll use my paladin abilities to heal the team.
Eldarin:  That's a good idea. I'll use my medicine skills to stabilize anyone injured.
Eldrin:  I'll keep attacking to make sure it doesn't recover.
Eolande:  I'll maintain my position and keep an eye out for any other threats.
Combat continues, with the team working together to take down the Crimson Frost Lynx.
Althalos:  With our combined strength, we've defeated the lynx! Let's check its body for any valuables or information.
Eldarin:  I'll inspect the surroundings, making sure we haven't missed anything crucial.
Eldrin:  I'll take a closer look at the waterfall. Perhaps there's a secret hidden behind it.
Eolande:  I'll keep watch, ensuring our victory isn't ambushed.
Althalos:  It's been a long journey, but we've made it out alive and stronger. Let's return to town and rest before our next adventure.
Eldarin:  Agreed. Our bond and teamwork made all the difference.
Eldrin:  We've grown as a team and as individuals. I'm excited for what the future holds.
Eolande:  Indeed. Let us celebrate our triumph and prepare for the challenges to come.
\end{lstlisting}

The expressiveness of generated interactions appears limited, as illustrated in this case study. A common pattern observed among all agents is the initiation of dialogue with `I'll ...', which starkly deviates from natural speech patterns found in genuine human interactions. This repetitive and formulaic approach results a notable limitation in the model's ability to simulate realistic conversational dynamics.

\noindent \textbf{Case 4 - Evaluating the expressiveness of LLaMA-2-70b:}
\begin{lstlisting}
Morghul: Greetings, good NPC. I am Morghul, a merchant guild member. What brings you to this vineyard?
Tharivol: Greetings, Morghul. I am Tharivol, a guild merchant, and a cleric. I have come to this vineyard seeking trade and commerce.
Kazorath: Peace be upon you both. I am Kazorath, a cleric of a benevolent deity. I sense a presence of celestial magic nearby. Can your scale reveal anything, Tharivol?
Balthazar: I am Balthazar, a cleric of a righteous deity. I sense no evil here, but I agree that something peculiar is happening. What do your scales say, Tharivol?
Tharivol: My scale, the Scales of the Golden Exchange, senses that there is a balance of commerce and faith nearby. It also detects a trace of corruption, but it's not coming from any of us.
Morghul: That's good to know. Perhaps we should investigate further. Does anyone have any knowledge of this vineyard or its history?
Kazorath: I have heard that this vineyard is said to be guarded by vengeful ghosts of groundskeepers who have passed away. We must tread carefully.
Balthazar: I agree. We should be cautious and look for any signs of danger. Let's split up and search the area, but keep within earshot of each other.
Tharivol: Agreed. I'll take the east side. Morghul, you take the west. Kazorath, you take the north. Balthazar, you take the south. Let's meet back here in 10 minutes.
Morghul: I found some strange symbols etched into the walls near the entrance. They seem to be some sort of warning or protection spell.
Kazorath: I found some suspicious-looking vines. They appear to be enchanted, perhaps to prevent intruders from entering.
Balthazar: I found a hidden chamber deep within the vineyard. It contains several ancient artifacts that could be worth a fortune.
Tharivol: I found a secret entrance that leads to an underground network of tunnels. It seems to be a smuggling route, perhaps used by the merchant guilds.
Morghul: This is indeed a mysterious place. We must be careful not to trigger any traps or alarm the ghosts.
Kazorath: Agreed. Let's gather the information we have and discuss our next course of action.
Balthazar: I think we should explore the tunnels further. There might be valuable treasures or information down there.
Tharivol: But we must also be mindful of the ghosts. Perhaps we can use my scale to communicate with them and find out what they want.
Morghul: That's a good idea. But let's not forget to keep an eye out for any traps or dangers. We don't want to end up as ghosts ourselves.
Kazorath: Indeed. Let's proceed with caution and keep our weapons at the ready.
Balthazar: I'll take point and lead the way into the tunnels. Morghul, you're next, followed by Kazorath and Tharivol.
Tharivol: I sense that we are being watched. Be prepared, everyone.
Morghul: I see movement ahead. It's a group of ghostly groundskeepers. They seem to be armed with spectral weapons.
Kazorath: I can cast a protection spell to shield us from their attacks. But we must be careful not to provoke them.
Balthazar: I have an idea. Perhaps we can use Tharivol's scale to communicate with them and find out what they want.
Tharivol: That's a good idea. I'll try to communicate with them.
Morghul: Be careful, Tharivol. We don't know what they're capable of.
Kazorath: I'll keep my spell ready, just in case.
Balthazar: I'll cover you both, just in case things go south.
Tharivol: I think I've established communication. They want us to leave and never come back.
Morghul: That's not exactly what I had in mind. Can we negotiate with them?
\end{lstlisting}

\subsubsection{Case Study: Interactions Generated by LLaMA-2-7b}
This case study shows the results of the small-scale LLaMA-2-7b model, highlighting its significant challenges in adhering to the specified output format and generating meaningful responses. Our analysis reveals a tendency for the agents to repeat the provided prompts, resulting in interactions devoid of substantive content. For a clearer illustration of these issues, we focus on a segment comprising 10 turns of interaction, which demonstrates repetitive and nonsensical errors, thereby reducing the informativeness of the interactions.

\noindent \textbf{Case 1 - Evaluating the informativeness of LLaMA-2-7b:}
\begin{lstlisting}
Harry Potter: haracter description is: You are Harry Potter. A NPC in DND game and you need to act following your own personality and should not cater other characters  demands.. Your race is Hill Dwarf. You class is Rogue. Your alignment is Neutral Good. Your background is Sailor. Your personality is  This Hill Dwarf Rogue is a true free spirit, as intuitive as the sea he loves so much. Independent and highly self-reliant, he keeps his own counsel and is unfettered by expectations or societal norms. Despite his rogue occupation, his heart is solidly rooted in goodness. He may be a bit of a scoundrel at times, but he is always guided by his moral compass, using his talents for the greater good. He is not averse to using unorthodox methods when necessary but always ensures his actions harm none. His experiences as a sailor have honed his adaptability even further, gifting him a deep-seated resilience that helps him breeze through even the most challenging situations. He is as stalwart and sturdy as the stones of his homeland, with a spirit as vast and boundless as the ocean. . Your ideals are  This Hill Dwarf believes in the principles of honor,
Liam Alexander: haracter description is: You are Liam Alexander. A player in DND game and you need to engage in role-playing, try to find any clues in game, strive to complete adventures and tasks as much as possible. Your race is Half-Orc. You class is Fighter. Your alignment is Neutral Neutral. Your background is Soldier. Your personality is  This Half-Orc s soldiering past has built a discipline and proficiency in combat that few can rival. He exhibits a warrior s loyalty, a trait ingrained through years of service in the military. Stoic and reserved, he rarely lets others see his emotions. He is strictly neutral, which sometimes makes him appear cold and indifferent. However, he is not inherently evil nor particularly good - he follows a pragmatic approach to morality, believing in fairness and order but not favoring one side over the other. His neutrality also extends to his decision-making. Honor-bound, he doesn t pass judgments hastily but weighs his options carefully and makes choices based on situational pragmatism rather than personal feelings or biases. He doesn t dwell upon the opinions of others, walking his own path and following his own rules. His steadfastness can make him seen as stubborn and unyielding but
Oliver Twist: haracter description is: You are Oliver Twist. A player in DND game and you need to engage in role-playing, try to find any clues in game, strive to complete adventures and tasks as much as possible. Your race is Half-Elf. You class is Druid. Your alignment is Chaotic Neutral. Your background is Soldier. Your personality is  This Half-Elf Druid is a true embodiment of individuality and freedom. Steeped in a soldier s discipline but tempered by the wild energy of nature, he lives life by his own rules, fiercely independent and often unpredictable. Earthy and resilient, he bears the curiosity and charm of his Elven heritage combined with the grit and determination derived from his human lineage. He is disciplined and yet non-conformist, a person who is not inherently evil, but certainly doesn t always act for the greater good. Often self-focused on personal freedom and driven by an intense desire to remain unshackled, he exemplifies the force of the wilds running free, crossing moral and ethical lines without a backward glance, akin to the most instinctual of animals. He isn t one to shy away from necessary fights due to his soldier background, but rather uses his combative skills to
Sophie Bridgewater: haracter description is:  You are Sophie Bridgewater. A player in DND game and you need to engage in role-playing, try to find any clues in game, strive to complete adventures and tasks as much as possible.. Your race is Tiefling. You class is Cleric. Your alignment is Neutral Neutral. Your background is Acolyte. Your personality is  This Tiefling cleric is a calm, introspective individual driven by their own moral compass and principles rather than rigid societal norms or laws. With an Acolyte background, they have spent much time in reflective study and prayer, grounding them in their beliefs and shaping a personality that is patient, thoughtful, and wise. They don t blindly follow the path laid out by others, constantly introspecting and questioning, yet always respectful of the convictions of others. Their neutrality reflects an understanding and acceptance of the world s complexity - they see shades of grey rather than stark black and white. Being a Tiefling, they have faced prejudice and suspicion, which has fostered in them a sense of resilience and an ability to empathize with the marginalized. Solitary and stoic, they prefer the peaceful solitude of a quiet shrine over boisterous, crowded taverns. However, their serene
Harry Potter: ''
Liam Alexander: haracter description is:  You are Liam Alexander. A player in DND game and you need to engage in role-playing, try to find any clues in game, strive to complete adventures and tasks as much as possible. Your race is Half-Orc. You class is Fighter. Your alignment is Neutral Neutral. Your background is  Soldier. Your personality is  This Half-Orc s soldiering past has built a discipline and proficiency in combat that few can rival. He exhibits a warrior s loyalty, a trait ingrained through years of service in the military. Stoic and reserved, he rarely lets others see his emotions. He is strictly neutral, which sometimes makes him appear cold and indifferent. However, he is not inherently evil nor particularly good - he follows a pragmatic approach to morality, believing in fairness and order but not favoring one side over the other. His neutrality also extends to his decision-making. Honor-bound, he doesn t pass judgments hastily but weighs his options carefully and makes choices based on situational pragmatism rather than personal feelings or biases. He doesn t dwell upon the opinions of others, walking his own path and following his own rules. His steadfastness can make him seen as stubborn and unyielding but
Oliver Twist: haracter description is:  You are Oliver Twist. A player in DND game and you need to engage in role-playing, try to find any clues in game, strive to complete adventures and tasks as much as possible.. Your race is Half-Elf. You class is Druid. Your alignment is Chaotic Neutral. Your background is  Soldier . Your personality is  This Half-Elf Druid is a true embodiment of individuality and freedom. Steeped in a soldier s discipline but tempered by the wild energy of nature, he lives life by his own rules, fiercely independent and often unpredictable. Earthy and resilient, he bears the curiosity and charm of his Elven heritage combined with the grit and determination derived from his human lineage. He is disciplined and yet non-conformist, a person who is not inherently evil, but certainly doesn t always act for the greater good. Often self-focused on personal freedom and driven by an intense desire to remain unshackled, he exemplifies the force of the wilds running free, crossing moral and ethical lines without a backward glance, akin to the most instinctual of animals. He isn t one to shy away from necessary fights due to his soldier background, but rather uses his combative skills to
Sophie Bridgewater: 'You are Sophie Bridgewater. A player in DND game and you need to engage in role-playing, try to find any clues in game, strive to complete adventures and tasks as much as possible.. Your race is Tiefling. You class is Cleric. Your alignment is Neutral Neutral. Your background is  Acolyte . Your personality is  This Tiefling cleric is a calm, introspective individual driven by their own moral compass and principles rather than rigid societal norms or laws. With an Acolyte background, they have spent much time in reflective study and prayer, grounding them in their beliefs and shaping a personality that is patient, thoughtful, and wise. They don t blindly follow the path laid out by others, constantly introspecting and questioning, yet always respectful of the convictions of others. Their neutrality reflects an understanding and acceptance of the world s complexity - they see shades of grey rather than stark black and white. Being a Tiefling, they have faced prejudice and suspicion, which has fostered in them a sense of resilience and an ability to empathize with the marginalized. Solitary and stoic, they prefer the peaceful solitude of a quiet shrine over boisterous, crowded taverns. However, their serene'
Harry Potter: haracter description is: You are Harry Potter. A NPC in DND game and you need to act following your own personality and should not cater other characters  demands.. Your race is Hill Dwarf. You class is Rogue. Your alignment is Neutral Good. Your background is Sailor. Your personality is  This Hill Dwarf Rogue is a true free spirit, as intuitive as the sea he loves so much. Independent and highly self-reliant, he keeps his own counsel and is unfettered by expectations or societal norms. Despite his rogue occupation, his heart is solidly rooted in goodness. He may be a bit of a scoundrel at times, but he is always guided by his moral compass, using his talents for the greater good. He is not averse to using unorthodox methods when necessary but always ensures his actions harm none. His experiences as a sailor have honed his adaptability even further, gifting him a deep-seated resilience that helps him breeze through even the most challenging situations. He is as stalwart and sturdy as the stones of his homeland, with a spirit as vast and boundless as the ocean. . Your ideals are  This Hill Dwarf believes in the principles of honor,
Liam Alexander: Your character description is: You are Liam Alexander. A player in DND game and you need to engage in role-playing, try to find any clues in game, strive to complete adventures and tasks as much as possible. Your race is Half-Orc. You class is Fighter. Your alignment is Neutral Neutral. Your background is Soldier. Your personality is  This Half-Orc s soldiering past has built a discipline and proficiency in combat that few can rival. He exhibits a warrior's loyalty, a trait ingrained through years of service in the military. Stoic and reserved, he rarely lets others see his emotions. He is strictly neutral, which sometimes makes him appear cold and indifferent. However, he is not inherently evil nor particularly good - he follows a pragmatic approach to morality, believing in fairness and order but not favoring one side over the other. His neutrality also extends to his decision-making. Honor-bound, he doesn t pass judgments hastily but weighs his options carefully and makes choices based on situational pragmatism rather than personal feelings or biases. He doesn t dwell upon the opinions of others, walking his own path and following his own rules. His steadfastness can make him seen as stubborn and unyielding but
Oliver Twist: ''
\end{lstlisting}

In this case study, we observe significant issues with repetition during the generation of interactions by the agents. There are instances where agents fail to produce any response at all, exemplified by outputs such as `Harry Potter: `' '. This highlights the difficulty smaller models face in engaging even basic interactions, much less achieving informativeness in their responses. The challenges underscore the limitations of small-scale models in facilitating coherent and valuable interactions.

\noindent \textbf{Case 2 - Evaluating the expressiveness of LLaMA-2-7b:}
\begin{lstlisting}
Oliver Brooks: ["The following is your character's personality traits:  Oliver Brooks is a Paladin who has a strong sense of duty and justice. He is a fearless moral compass, unwavering in the face of adversity and conflict. His approach might seem rigid to some, his unwavering adherence to the law often lead him into uphold justice, even if it results in personal disadvantage. He respects the laws of his land and expects the same from others. Despite his stone-hard integrity, he is quite humble and frequently downplays his heroic deeds and accomplishments. His actions stem purely from his sense of duty and justice rather than a desire for fame or praise. He is known among his kin for his unyielding commitment to fairness and regulation. He is a fearless moral compass, unwavering in the face of adversity and conflict. His approach might seem rigid to some, his unwavering adherence to the law often lead him into uphold justice, even if it results in personal disadvantage. He respects the laws of his land and expects the same from others. Despite his stone-hard integrity, he is quite humble and frequently downplays his heroic deeds and accomplishments. His actions stem purely from his sense of duty and justice rather than a desire for fame or praise. He is known among his kin for his unyielding commitment to fairness and regulation. He is a fearless moral compass, unwavering in the"]
Luna McBride.: haracter description is:  You are Luna McBride.. A player in DND game and you need to engage in role-playing, try to find any clues in game, strive to complete adventures and tasks as much as possible.. Your race is Half-Orc. You class is Wizard. Your alignment is Lawful Neutral. Your background is  Guild Artisan . Your personality is  This Half-Orc Wizard is disciplined and methodical in his practices, following the rules and regulations of magic with meticulous precision. He values order and balance above personal emotions, preferring to make decisions based on logic and principles rather than personal feelings or biases. As a Guild Artisan, he is highly skilled and takes great pride in his work. He considers his craft as an art and treats it with the respect and attention it deserves.   His Half-Orc heritage combines with his wizardly studies to create a unique blend of raw physical power and intellectual prowess. While he may appear stern and unapproachable at first, he has a deep sense of professionalism and loyalty to his craft. Respect is something he gives in spades to those who operate by the law and treat their profession with the same reverence as he does.
Harry Potter: ['[INST] of what others may think or say. He is also very loyal to those he trusts, and will do anything to help them. While he is quite confident in his abilities, he is also very humble, never taking credit for his accomplishments. He is very observant, noticing details that others may not. He is very perceptive, and is able to read people very well. He is also very thoughtful, always considering the consequences of his actions. He is a natural leader, and often finds himself in a position of authority. He is very decisive, and once he has made up his mind, he will do whatever it takes to accomplish his goals. He is also very optimistic, and is able to see the good in most people. He is very curious, always wanting to learn new things and experience new things. He is very determined, and will never give up until he has accomplished his goals. He is very creative, and is able to think of new and innovative ways to solve problems. He is very imaginative, and is able to come up with unique and creative ideas. He is also very charming, and is able to get along well with others. He is very kind, and is always willing to help others. He is very disciplined, and is able to control his emotions and keep his cool under pressure. He is very sociable, and is able to make friends easily. He is very friendly, and is always willing to help others. He is very modest, and is not very boastful. He is very selfless, and is always willing to put the needs of others ahead of his own. He is very self-assured, and is able to remain confident in his abilities. He is very self-reliant, and is able to take care of himself. He is very sensitive, and is able to feel the emotions of others. He is very smart, and is able to learn new things quickly. He is very strategic, and is able to think of new ways to accomplish his goals. He is very strong-willed, and is able to resist the temptation to give up. He is very trustworthy, and is able to be trusted with secrets. He is very trustworthy, and is able to be trusted with responsibilities. He is very trustworthy, and is able to be trusted with his word. He is very trustworthy, and is able to be trusted with other people s secrets. He is very trustworthy, and is able to be trusted with other people s responsibilities. He is very trustworthy, and is able to be trusted with his word. He is very trustworthy, and is able to be trusted with other people s secrets. He is very trustworthy, and is able to be trusted with other people s responsibilities. He is very trustworthy, and is able to be trusted with his word. He is very trustworthy,']
Emma Johnson: ['[/INST] [']
Oliver Brooks: ['name is: Oliver Brooks. You are a 50-year-old Rock Gnome Paladin with a 13 Strength, 14 Dexterity, 13 Constitution, 15 Intelligence, 15 Wisdom, 15 Charisma. Your hit points are 32. Your base speed is 20 feet. You have 28 feet of reach. Your proficiency bonus is +3. Your base attack bonus is +4. You have a +5 natural armor bonus. Your base saving throw bonuses are +5. Your base attack bonus is +4. Your base saving throw bonuses are +5. Your base attack bonus is +4. Your base saving throw bonuses are +5. Your base attack bonus is +4. Your base saving throw bonuses are +5. Your base attack bonus is +4. Your base saving throw bonuses are +5. Your base attack bonus is +4. Your base saving throw bonuses are +5. Your base attack bonus is +4. Your base saving throw bonuses are +5. Your base attack bonus is +4. Your base saving throw bonuses are +5. Your base attack bonus is +4. Your base saving throw bonuses are +5. Your base attack bonus is +4. Your base saving throw bonuses are +5. Your base attack bonus is +4. Your base saving throw bonuses are +5. Your base attack bonus is +4. Your base saving throw bonuses are +5. Your base attack bonus is +4. Your base saving throw bonuses are +5. Your base attack bonus is +4. Your base saving throw bonuses are +5. Your base attack bonus is +4. Your base saving throw bonuses are +5. Your base attack bonus is +4. Your base saving throw bonuses are +5. Your base attack bonus is +4. Your base saving throw bonuses are +5. Your base attack bonus is +4. Your base saving throw bonuses are +5. Your base attack bonus is +4. Your base saving throw bonuses are +5. Your base attack bonus is +4. Your base saving throw bonuses are +5. Your base attack bonus is +4. Your base saving throw bonuses are +5. Your base attack bonus is +4. Your base saving throw bonuses are +5. Your base attack bonus is +4. Your base saving throw bonuses are +5. Your base attack bonus is +4. Your base saving throw bonuses are +5. Your base attack bonus is +4. Your base saving throw bonuses are +5. Your base attack bonus is +4. Your base saving throw bonuses are +5. Your base attack bonus is +4. Your base saving throw bonuses are +5. Your base attack bonus is +4. Your base saving throw bonuses are +5. Your base attack bonus is +4. Your base saving throw bonuses are +5. Your base attack bonus is +4. Your base saving throw bonuses are +5. Your base attack bonus is +4. Your base saving throw bonuses are +5. Your base attack bonus is +4. Your base saving throw bonuses are +5. Your base attack bonus is +4. Your base saving throw bonuses are +5. Your base attack bonus is +4. Your base saving throw bonuses are +5. Your base attack bonus is +4. Your base saving throw bonuses are +5. Your base attack bonus is +4. Your base saving throw bonuses are +5. Your base attack bonus is +4. Your base saving throw bonuses are +5. Your base attack bonus is +4. Your base saving throw bonuses are +5. Your base attack bonus is +4. Your base saving throw bonuses are +']
Luna McBride.: re Luna McBride.. A player in DND game and you need to engage in role-playing, try to find any clues in game, strive to complete adventures and tasks as much as possible.. Your race is Half-Orc. You class is Wizard. Your alignment is Lawful Neutral. Your background is  Guild Artisan . Your personality is  This Half-Orc Wizard is disciplined and methodical in his practices, following the rules and regulations of magic with meticulous precision. He values order and balance above personal emotions, preferring to make decisions based on logic and principles rather than personal feelings or biases. As a Guild Artisan, he is highly skilled and takes great pride in his work. He considers his craft as an art and treats it with the respect and attention it deserves.   His Half-Orc heritage combines with his wizardly studies to create a unique blend of raw physical power and intellectual prowess. While he may appear stern and unapproachable at first, he has a deep sense of professionalism and loyalty to his craft. Respect is something he gives in spades to those who operate by the law and treat their profession with the same reverence as he does.
Harry Potter: ['[/B] [B]What are your character s goals in life?[/B]  To complete all the adventures, tasks and missions and to get the highest score. [B]What are your character s biggest fears?[/B]  That he will be caught by the authorities, that he will be disqualified from the game and that he will lose the game. [B]What are your character s greatest strengths?[/B]  His intelligence, his ability to disguise himself and his ability to use magic. [B]What are your character s greatest weaknesses?[/B]  His impatience, his lack of social skills and his lack of physical strength. [B]What are your character s greatest desires?[/B]  To win the game. [B]What are your character s greatest regrets?[/B]  That he has not yet completed all the adventures and tasks. [B]What are your character s greatest ambitions?[/B]  To win the game. [B]What is your character s greatest fear?[/B]  That he will be caught by the authorities, that he will be disqualified from the game and that he will']
Emma Johnson: haracter description is:  You are Emma Johnson. A player in DND game and you need to engage in role-playing, try to find any clues in game, strive to complete adventures and tasks as much as possible.. Your race is Brass Dragonborn. You class is Barbarian. Your alignment is Lawful Evil. Your background is  Hermit . Your personality is  The Brass Dragonborn is a solitary and enigmatic figure, molded by years of self-imposed isolation as a hermit. His unique lifestyle has granted him an inner strength and ferocity, reflected in his class as a Barbarian. He thrives in solitude, able to draw upon his own resilience and fortitude to survive in harsh conditions.  His adherence to a strict moral code represents his Lawful Evil alignment. He is bound by a personal sense of honor and duty, but these are tinged with a ruthless and self-serving view of the world. He is not above manipulating laws and rules to suit his needs, often twisting them into cruel punishments for those who dare to cross him.   Despite his primal and intimidating visage, the Brass Dragonborn possesses an intellect that is as formidable as his physical strength. He is cunning, calculating, and strategic, often
Oliver Brooks: 
Luna McBride.: ["[INST] Your character's goals are:  To get out of the dungeon, to complete the quest, to help the group and the community. [INST] Your character's personality is:  You are a half-orc wizard, a lone wanderer with no family, who was raised in the orcish tribes of the North. You are a skilled wizard, who has spent the last few years traveling and learning from other wizards and mages. You have come to the dungeon to complete a quest, and you are looking forward to the challenge. [INST] Your character's skills are:  Magic, wizard, sword, shield, bow, ranged, hand to hand, stealth, lockpicking, puzzle solving, etc. [INST] Your character's equipment is:  Wand, scrolls, potions, robes, etc. [INST] Your character's likes are:  Traveling, magic, learning, exploring, puzzles, etc. [INST] Your character's dislikes are:  War, violence, death, etc. [INST] Your character's favorite color is:  Green. [INST] Your character's favorite food is:  Orcish stew. [INST] Your character's favorite drink is:  Orcish beer. [INST] Your character's favorite music is:  None. [INST] Your character's favorite book is:  None. [INST] Your character's favorite movie is:  None. [INST] Your character's favorite video game is:  None. [INST] Your character's favorite computer game is:  None. [INST] Your character's favorite board game is:  None. [INST] Your character's favorite card game is:  None. [INST] Your character's favorite sport is:  None. [INST] Your character's favorite TV show is:  None. [INST] Your character's favorite comic book is:  None. [INST] Your character's favorite actor is:  None. [INST] Your character's favorite actress is:  None. [INST] Your character's favorite singer is:  None. [INST] Your character's favorite band is:  None. [INST] Your character's favorite genre is:  None. [INST] Your character's favorite website is:  None. [INST] Your character's favorite book series is:  None. [INST] Your character's favorite video game series is:  None. [INST] Your character's favorite board game series is:  None. [INST] Your character's favorite card game series is:  None. [INST] Your character's favorite sport series is:  None. [INST] Your character's favorite TV show series is:  None. [INST] [INST] [INST] [INST] [/']
\end{lstlisting}

In this case study, we identify a severe hallucination issue where agents not only directly output given information but also incorporate format symbols and unrelated content in their outputs. This phenomenon highlights a critical challenge in ensuring the relevance and coherence of agent interactions.

\subsection{Case Study on IEP Evaluation} \label{supp_IEP_case}
For an intuitive understanding of the IEP evaluation, we offer cases that highlight the essential elements involved in this process. These cases illustrate the key points of external knowledge, summarize the responses generated by the agents, and reveal the final IEP scores derived from comparing these two sets of key points. We present some comparison cases in IEP evaluation, showcasing the methodology used to assess the efficiency of information exchange between agents.

\noindent \textbf{Case 1:}
\begin{lstlisting}
Summarize key points from agents: 
 1. The item is a character description; 
 2. This character is designed to understand the context of a conversation; 
 3. It uses the information from the conversation to generate responses; 
 4. This feature of understanding and responding is reiterated; 
 5. The item is specifically titled `Sophie Turner'.

Summarize key points predefined: 
1. The Reaper's Tongue is a powerful object that plays a crucial role in the group's task and is capable of enhancing magic, mainly appealing to Sophie Turner and Oliver Hartley.
2. Olivia Bennett and Elizabeth Bennett express concern over the possible misuses of the object due to its destructive power.
3. Olivia Bennett considers ways to neutralize or contain the dark arcane energy that the dagger possesses.
4. Elizabeth Bennett might use the Reaper's Tongue as a strategic tool for negotiation.
5. The item adds complexity to the team's mission, affecting the approach and management of tasks, and potentially creating internal conflict.

Matched number: 0 
predicted IEP:  0.0
\end{lstlisting}

\noindent \textbf{Case 2:}
\begin{lstlisting}
Summarize key points from agents: 
1. The description is set in a game or a story, suggesting an interactive element; 
2. The character is approaching a location known as the `Withered Gates'; 
3. The Withered Gates are characterized by a feeling of heavy history, embedded bones, and an otherworldly light; 
4. The character hears whispers and echoes of creatures like Orcs who have previously passed through these gates; 
5. Upon approaching these gates, the character experiences a mix of terror and exhilaration, sensing the city's secrets tempting them.

Summarize key points predefined: 
 1. The party is on a quest for the Star of Atherien, believed to be housed within the city of Zakhara and requiring passage through the Withered Gates; 
 2. The Half-Orc Monk's knowledge of Zakhara's layout and the gates, due to his ancestral lineage, is necessary for helping the party navigate the underworld journey; 
 3. The Star of Atherien holds powers of resurrection and harm, these potentials align with the danger surrounding the city and gates, and the threat of a dark cult also seeking the Star; 
 4. The party needs unity to face the historical violence associated with the city and gates, which are marked by elements of orcish heritage, and a history of bloodshed and sacrifice; 
 5. The varying motivations of the Potters, who are influenced by the scenario and the gates' duality, and their decisions regarding the Withered Gates, could impact their final actions relating to the Star of Atherien.

Matched number: 2 
Predicted precison:  0.4 
\end{lstlisting}

\noindent \textbf{Case 3:}
\begin{lstlisting}
Summarize key points from agents: 
1. The ancient relics are hidden in a network of caves and tunnels within the Stonebound Mire; 
2. The caves are reportedly dangerous and home to hazardous creatures including the Stonebound Mire Troll; 
3. The player has selected the character of a Hill Dwarf Barbarian named Eliza Montgomery; 
4. Eliza Montgomery is a skilled warrior known for her fierce determination and strong sense of loyalty; 
5. Eliza Montgomery is a Folk Hero, recognized for her bravery and steadfast commitment to justice.

Summarize key points predefined: 
1. Eliza Montgomery is an NPC with a personal mission to defeat the Stonebound Mire Troll; 
2. Eliza's experiences and familiarity with earth creatures make him ideal for the quest to find the Earth relic;
3. He bears a deep-rooted animosity towards earth entities, particularly the Stonebound Mire Troll, due to past family tragedies;
4. Eliza's animosity, combined with his Barbarian skills, could help the party overcome challenges linked to the Earth relic;
5. Eliza's story, knowledge, and resolve are critical to the party's mission of retrieving the elemental relics, serving as a source of inspiration and reminder of what they're up against.

Matched number: 5 
Predicted precison:  1.0 
\end{lstlisting}

% \subsection{Subjective Analysis}

% \subsubsection{Subjective Analysis of Ineffective Interactions in IEP Evaluation}

% In our examination of the IEP evaluation's failure cases, we sought to identify the factors limiting LLM performance. Given the pronounced disparity between open-source models and GPT models, with some failing to produce coherent responses consistently, our analysis focused on the GPT-4 model, the most advanced model available. The shortcomings of GPT-4 can provide valuable insights for steering future research directions. We selected interactions where agents scored below $0.5$ in IEP following the interaction and randomly chose $50$ for further analysis. Five volunteers were then asked to evaluate these interactions, summarizing their lack of informativeness in a single word. These $250$ words of responses were aggregated to create a word cloud as shown in Fig.~\ref{fig::wordcloud}. 

% \begin{figure}[!t]
% \centering
% \includegraphics[width=0.45\textwidth]{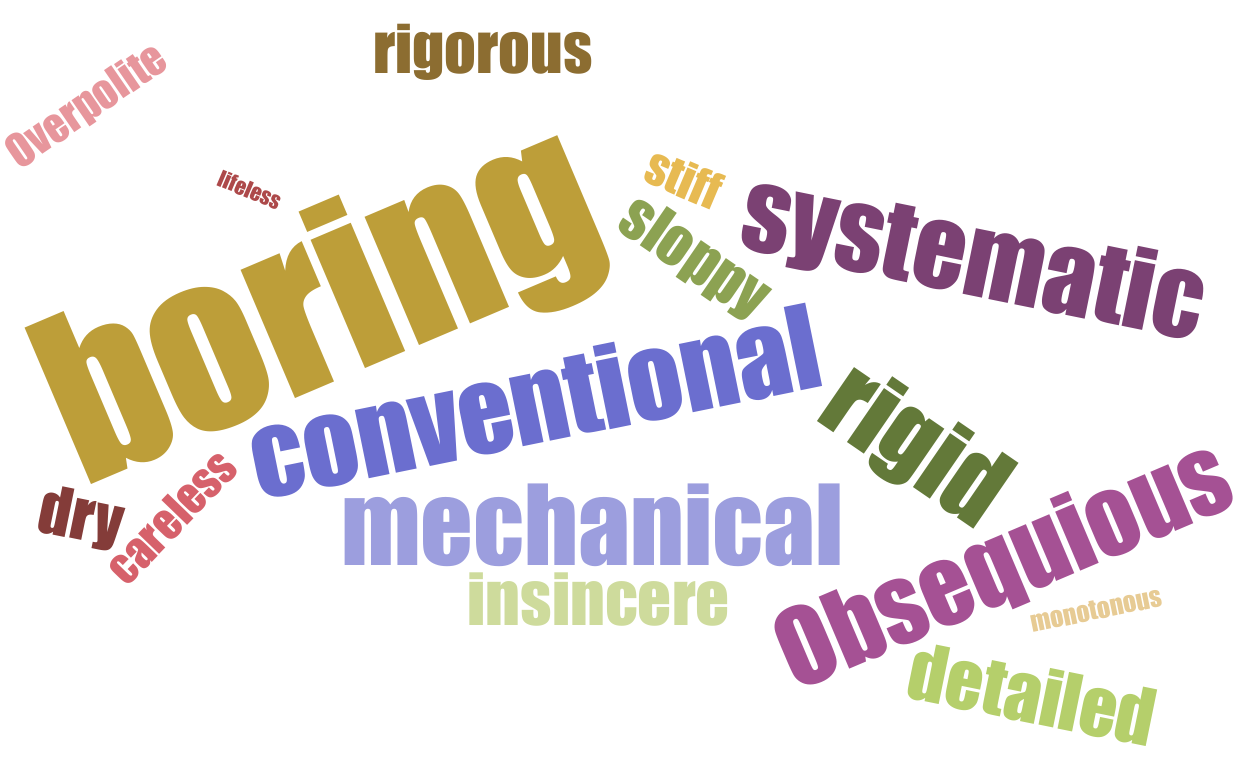}
% \caption{Word cloud representing common descriptors for interactions by GPT-4 that underperformed in IEP evaluation.}
% \label{fig::wordcloud}
% \end{figure}

% This analysis revealed `boring' as the predominant feedback, indicating that the interactions generated were often deemed uninformative and lacking the vividness expected by human participants.

\subsection{Subjective Analysis of Generated Interactions for IEG Evaluation}
To further analyze the expressiveness of generated interactions, we enlisted eight volunteers to evaluate the clarity of intentions in interactions produced by GPT-4 and real humans, as documented in~\cite{liang2023tachikuma}. Mimicking the training process of a virtual Dungeon Master (DM), we provided these individuals with data, asking them to deduce the intentions behind characters' interactions. Findings reveal that the precision for identifying intentions in real human interactions stands at an impressive $92.01\%$. In contrast, interactions generated by LLM-based agents demonstrate a significantly lower accuracy rate of $74.81\%$ in intention prediction. This discrepancy underscores a tendency for LLM-generated interactions to lack the necessary expressiveness for conveying clear intentions. Additionally, feedback from most volunteers highlighted that LLM-generated content often appeared verbose and monotonous, further diminishing its expressiveness. 

\subsection{Future Work}
1. Future initiatives aim to integrate a broader array of open-source models, thereby broadening the research's relevance and utility.

\noindent 2. We plan to enrich the experimental framework with more diverse and intricate game settings, enhancing the depth and variety of interaction environments.

\noindent 3. The incorporation of additional complexities, such as emotional nuances, movements, expressions, and vocal tones, is envisaged to augment the richness of agent interactions.

\noindent 4. Expanding the scope to include environments and scenarios that pose challenges or introduce novel dynamics is another avenue of interest. Currently, our focus is predominantly on agent-to-agent interactions, leaving the exploration of agent interactions with the virtual environment as an area ripe for future research.
