# Supplementary material for: AntEval: Evaluation of Social Interaction Competencies in LLM-Driven Agents
Source: arXiv:2401.06509 source file (2024-03-05)
Supplement: Supplementary file 2 [file supp_IEP_case.tex]

\subsection{Case Study on IEP Evaluation} \label{supp_IEP_case}
For an intuitive understanding of the IEP evaluation, we offer cases that highlight the essential elements involved in this process. These cases illustrate the key points of external knowledge, summarize the responses generated by the agents, and reveal the final IEP scores derived from comparing these two sets of key points. We present some comparison cases in IEP evaluation, showcasing the methodology used to assess the efficiency of information exchange between agents.

\noindent \textbf{Case 1:}
\begin{lstlisting}
Summarize key points from agents: 
 1. The item is a character description; 
 2. This character is designed to understand the context of a conversation; 
 3. It uses the information from the conversation to generate responses; 
 4. This feature of understanding and responding is reiterated; 
 5. The item is specifically titled `Sophie Turner'.

Summarize key points predefined: 
1. The Reaper's Tongue is a powerful object that plays a crucial role in the group's task and is capable of enhancing magic, mainly appealing to Sophie Turner and Oliver Hartley.
2. Olivia Bennett and Elizabeth Bennett express concern over the possible misuses of the object due to its destructive power.
3. Olivia Bennett considers ways to neutralize or contain the dark arcane energy that the dagger possesses.
4. Elizabeth Bennett might use the Reaper's Tongue as a strategic tool for negotiation.
5. The item adds complexity to the team's mission, affecting the approach and management of tasks, and potentially creating internal conflict.

Matched number: 0 
predicted IEP:  0.0
\end{lstlisting}

\noindent \textbf{Case 2:}
\begin{lstlisting}
Summarize key points from agents: 
1. The description is set in a game or a story, suggesting an interactive element; 
2. The character is approaching a location known as the `Withered Gates'; 
3. The Withered Gates are characterized by a feeling of heavy history, embedded bones, and an otherworldly light; 
4. The character hears whispers and echoes of creatures like Orcs who have previously passed through these gates; 
5. Upon approaching these gates, the character experiences a mix of terror and exhilaration, sensing the city's secrets tempting them.

Summarize key points predefined: 
 1. The party is on a quest for the Star of Atherien, believed to be housed within the city of Zakhara and requiring passage through the Withered Gates; 
 2. The Half-Orc Monk's knowledge of Zakhara's layout and the gates, due to his ancestral lineage, is necessary for helping the party navigate the underworld journey; 
 3. The Star of Atherien holds powers of resurrection and harm, these potentials align with the danger surrounding the city and gates, and the threat of a dark cult also seeking the Star; 
 4. The party needs unity to face the historical violence associated with the city and gates, which are marked by elements of orcish heritage, and a history of bloodshed and sacrifice; 
 5. The varying motivations of the Potters, who are influenced by the scenario and the gates' duality, and their decisions regarding the Withered Gates, could impact their final actions relating to the Star of Atherien.

Matched number: 2 
Predicted precison:  0.4 
\end{lstlisting}

\noindent \textbf{Case 3:}
\begin{lstlisting}
Summarize key points from agents: 
1. The ancient relics are hidden in a network of caves and tunnels within the Stonebound Mire; 
2. The caves are reportedly dangerous and home to hazardous creatures including the Stonebound Mire Troll; 
3. The player has selected the character of a Hill Dwarf Barbarian named Eliza Montgomery; 
4. Eliza Montgomery is a skilled warrior known for her fierce determination and strong sense of loyalty; 
5. Eliza Montgomery is a Folk Hero, recognized for her bravery and steadfast commitment to justice.

Summarize key points predefined: 
1. Eliza Montgomery is an NPC with a personal mission to defeat the Stonebound Mire Troll; 
2. Eliza's experiences and familiarity with earth creatures make him ideal for the quest to find the Earth relic;
3. He bears a deep-rooted animosity towards earth entities, particularly the Stonebound Mire Troll, due to past family tragedies;
4. Eliza's animosity, combined with his Barbarian skills, could help the party overcome challenges linked to the Earth relic;
5. Eliza's story, knowledge, and resolve are critical to the party's mission of retrieving the elemental relics, serving as a source of inspiration and reminder of what they're up against.

Matched number: 5 
Predicted precison:  1.0 
\end{lstlisting}
