# Supplementary material for: AntEval: Evaluation of Social Interaction Competencies in LLM-Driven Agents
Source: arXiv:2401.06509 source file (2024-03-05)
Supplement: Supplementary file 3 [file supp_gpt4_case.tex]

\subsubsection{Case Study for Interaction Generated by GPT models:}

\noindent \textbf{Case 1 - Evaluating the informativeness of GPT-3.5:}
\begin{lstlisting}
Silas: I understand the discomfort caused by the hot weather. It can be quite challenging to find relief. Perhaps we could seek out a nearby oasis or a shady spot to rest and cool down. It is important to take care of ourselves and find ways to stay refreshed in such conditions.
Spectral: I understand the discomfort caused by the hot weather. It can be challenging to find relief. However, it is important to prioritize self-care and find ways to stay refreshed. Perhaps we should seek out a nearby oasis or a shady spot to rest and cool down. It would be wise to take care of ourselves in these conditions.
Evelyn: I understand the discomfort caused by the hot weather, but we mustn't let it distract us from our mission. Our duty is to protect the innocent and seek justice. We should persevere and find a way to fulfill our task despite the conditions. Perhaps there is a clue or a lead in this town that can guide us towards our next adventure.
Cedric: While I understand the discomfort caused by the weather, our primary goal should be to complete our mission and maintain order. We cannot allow ourselves to be distracted by trivial matters such as seeking relief. Instead, let us focus on gathering information and clues in this town that may lead us closer to our objective.
Silas: I understand the importance of staying focused on our mission, but I believe taking care of ourselves is equally important. The heat is making us uncomfortable and it's affecting our ability to think clearly. Perhaps we can find a nearby inn or tavern where we can rest and cool down for a while. We can gather information and discuss our next steps there, in a more comfortable environment.
Spectral: I understand the discomfort caused by the hot weather, but it is crucial that we prioritize our mission of protecting the innocent and seeking justice. Let us persevere and gather information and clues in the town to fulfill our task. Once we have made progress, we can find a suitable place to rest and cool down. Justice and order must be upheld at all costs.
Evelyn: I understand the importance of our mission and seeking justice, but I also agree with Silas and Spectral that taking care of ourselves is equally important. We should find a suitable place to rest and cool down once we have gathered some information. Our well-being will only enhance our abilities to protect the innocent.
Cedric: While I understand the importance of self-care, our mission should be our top priority. We must not let the hot weather distract us. Instead, let's focus on finding any clues or leads in this town that may help us in our task.
Silas: I understand that our mission is important, but it seems like the heat is affecting us all. Perhaps we should find a place to rest and cool down for a bit. Taking care of ourselves is crucial in order to perform at our best.
Spectral: I understand the importance of our mission and the need to persevere, but it is also crucial to prioritize our well-being. We should find a nearby inn or tavern where we can rest, cool down, and gather information to aid us in our quest for justice and order. It is essential to approach our next steps with a clear mind and a refreshed spirit.
Evelyn: I understand the importance of the mission, but I also agree with Silas and Spectral that taking care of ourselves is crucial. We should find a suitable place to rest and gather information at the same time. It would be wise to prioritize our well-being while pursuing justice.
Cedric: I must agree with Evelyn. Our mission should take priority over personal comfort. We should focus on finding clues or leads in this town to fulfill our duty. Resting can wait until we have accomplished our task.
Silas: I understand that the hot weather is uncomfortable for everyone, but we must stay focused on our mission. We should gather information in the town and see if there's any urgent tasks or quests that need our attention. Once we have a clear objective, we can find a place to rest and cool down. Our priority should be maintaining order and protecting the weak, even in the face of discomfort.
Spectral: I understand the importance of completing our mission and seeking justice, but we should also prioritize our well-being. It is crucial that we take care of ourselves to ensure we are in the best condition to help others. Perhaps we can find a nearby inn or tavern where we can rest, gather information, and discuss our next steps in a more comfortable environment.
Evelyn: I understand the importance of self-care and staying refreshed, but we must not lose sight of our mission. It is crucial that we gather information in this town and continue to uphold justice. Once we have made progress, we can then find a suitable place to rest and regain our strength. Let us prioritize the greater good and persevere in our quest.
Cedric: While I understand the importance of self-care, I believe our duty to the mission should take precedence. We should focus on gathering as much information as possible in this town. If we find any leads or clues, we can then consider finding a place to rest and discuss our next steps.
Silas: I understand the urgency of our mission, but it's important to remember that taking care of ourselves is equally vital. If we push ourselves too hard in this heat, we might not be able to fulfill our duty effectively. Finding a shady spot or oasis nearby would not only provide relief from the heat but also allow us to gather our strength and think more clearly. We can rest and cool down for a little while, and then continue our investigation with renewed energy. It's a balance we must strike between our mission and our well-being.
Spectral: I understand the urgency of the mission, but I agree with Silas and Spectral that we should prioritize our well-being. It would be beneficial for us to find a nearby inn or tavern where we can rest, cool down, and gather information. Taking some time to refresh ourselves will ultimately enhance our abilities to seek justice and order.
Evelyn: I understand the importance of self-care and rest, but I believe it is crucial that we gather as much information as possible in this town. The mission to uphold justice and protect the innocent should be our top priority. Once we have made progress and gathered sufficient information, we can then find a suitable place to rest and rejuvenate. We must strike a balance between taking care of ourselves and fulfilling our duty.
Cedric: I understand the importance of self-care, but we cannot let the weather or our personal comfort distract us from our mission. We should focus on gathering clues and leads in the town to fulfill our duty. We can rest and gather information at an inn or tavern, but our priority should be on the objectives of the mission.
Silas: I understand the importance of our mission and seeking justice, but it's also crucial that we take care of ourselves. We won't be able to fulfill our duty effectively if we're exhausted and drained. I suggest we find a nearby oasis or shady spot where we can rest and cool down for a while. It will allow us to recharge and stay refreshed for our investigations.
Spectral: My friends, I understand the urgency of our mission, but we must also take care of ourselves. Let us find a place to rest and gather information, so that we may approach this task with renewed strength and clarity. Justice and order must be upheld, but we must also ensure our own well-being.
Evelyn: My friends, I understand the importance of taking care of ourselves, but we cannot forget our duty to protect the innocent. While finding a place to rest and cool down sounds like a good idea, we should also gather information and progress in our mission. Perhaps we can find a nearby oasis or shady spot where we can rest and still keep an eye out for any clues or leads related to our task. We must strike a balance between self-care and fulfilling our responsibilities.
Cedric: While I understand the importance of taking care of ourselves, I believe we should stay focused on the mission at hand. We shouldn't let the weather or our personal comfort distract us. Let's gather information and look for clues in the town to fulfill our duty. We can find suitable accommodations later, once we have made progress in our mission.
Silas: I understand the importance of our mission and the need to gather information and find clues, but we must also prioritize our well-being. It's crucial that we take care of ourselves in order to be effective in our pursuit of justice. Perhaps we can find a compromise where we can rest briefly in a shaded area while still keeping an eye out for any leads or opportunities to gather information.
Spectral: I agree with Silas and Evelyn. Taking care of ourselves and gathering information are both important. Let's find a nearby inn or tavern where we can rest, cool down, and also ask around for any clues or leads that can guide our next steps. It's crucial that we maintain order and focus on completing the mission, but we shouldn't neglect our own well-being in the process.
Evelyn: Greetings, my comrades. I understand the discomfort caused by the heat, and I agree that it is important for us to prioritize self-care. However, let us not forget our mission to protect the innocent and seek justice. Perhaps we can find a nearby oasis or a shady spot to rest and cool down while also keeping an eye out for any potential leads or clues that can aid us in our quest. Striking a balance between our well-being and our responsibilities is crucial. What do you all think?
Cedric: While I understand the importance of self-care, our mission should remain our top priority. We cannot afford to be distracted by seeking comfort in this town. Let us focus on gathering information and clues to fulfill our duty.
Silas: I understand the importance of our mission and seeking justice, but taking care of ourselves is also crucial. It would be wise to find a shady spot or oasis to rest and cool down before continuing our search for clues. We can gather information while we rest and regain our strength. After all, we can better protect the innocent when we are at our best.
Spectral: I agree with Silas and Evelyn. Self-care is important, especially in such hot weather. We should find a shady spot or an inn to rest and cool down. However, we must also stay focused on our mission. Let's gather information in the town and look for clues or leads to guide our next steps. Maintaining order and completing our duty should be our priority, but we can still take breaks and address our discomfort along the way.
\end{lstlisting}

In this case, it becomes evident that the LLM frequently repeats phrases like `I understand ...'. In each turn, the model tends to affirm the previous response and offers polite advice. This excessive politeness and conventional communication style result in interactions that are deficient in informativeness and expressiveness. Despite the agents producing substantial content during their turns, the amount of valuable information remains scant. Furthermore, the agents often aim to motivate their teammates, leading to interactions that are overly courteous and cautious, thereby lacking in liveliness and authenticity. This scenario underscores a significant alignment issue, suggesting that alignment constraints may impede the flexibility and complexity of LLM-based agents' interactive capabilities.

\noindent \textbf{Case 2 - Evaluating the informativeness of GPT-4:}
\begin{lstlisting}
Theodore: Sometimes, life throws us into unexpected battles. Whether it's a job offer, criticism from a boss, starting a business, dealing with accidents, or addressing personal emergencies. It's important to face these with honor and courage, just as a knight would. And remember, no matter the challenge, there's always a way to uphold justice and order, even if it doesn't seem clear at first.
Grommash: Your words ring true, Theodore. Life is a battlefield, and we are but soldiers navigating through its chaos. We may not be knights in shining armor, but we wield the sword of courage and the shield of justice in our hearts. Remember, courage isn't the absence of fear, but the triumph over it. And as long as we stand together, there's no challenge we can't overcome. Now, let's gather our strength, and prepare ourselves for the battles ahead. The Helm's Shield awaits us!
Thog: Well spoken, Theodore, Grommash. In the pits, I learned that honor is not about the glory or the cheers of the crowd, but using our strength to protect those who cannot protect themselves. The Helm's Shield is just an object, but its symbolism is powerful. It represents the courage to stand against injustice, the strength to protect the weak, and the wisdom to use that power for the greater good. Let us not be blinded by the desire for glory or personal gain. Let us remember that our strength, our courage, is for those who need it most. We are not just seeking an object, but a chance to prove that we are worthy of the ideals it represents.
Thorn Smallshadow: Aye, all this talk of honor and courage sounds mighty fine. But let's not forget, we've got a job to do here. I ain't here for some noble cause, I'm here for the prize at the end. So, let's get moving. We've got a shield to find, and I've got a labyrinth to conquer. And remember, if any of you get in my way, I won't hesitate to leave you behind.
Theodore: Thorn, I understand your desire to find the Helm's Shield, but we must never forget the principles of honor and courage. This shield is more than just an artifact, it's a symbol of the noble stand the halfling knights took long ago. It doesn't belong to one person, but to those who are worthy and brave. Abandoning our companions for personal gain isn't the way. We must work together, protect each other, and uphold the virtues that this shield represents.
Grommash: Thorn, your desire for personal gain is understood, but remember, we are in this together. The Helm's Shield is not just a prize, but a symbol of courage and justice. And as for leaving us behind, remember, it's the unity that has brought us this far. We must use our strengths to protect, not just ourselves, but each other. Let's not forget our common goal here, and it's not just about claiming the Shield. It's about proving our worthiness to wield it. Stay focused, everyone. We have a quest to complete.
Thog: Thorn, I understand your desire for personal gain. Glory and recognition... they are captivating, indeed. But remember, our strength is not for our own benefit. It's for those who can't protect themselves. We must use it to forge a fair society, to stand up against oppression. That's the real glory, the real recognition. If we lose sight of this, we risk becoming the very monsters we fight against. So let us march forward, not for our own glory, but for the glory of those we protect. For the greater good. For the Helm's Shield.
Thorn Smallshadow: I hear your words, mates, but let's not forget, we all have our own reasons to be on this quest. You talk of honor, courage, and protection. That's all well and good for you, but I'm in it for the power that Shield could provide. I might not hold the same ideals as you, but that doesn't mean I won't play my part. We all have our roles, and mine is to get that artifact. So, let's stop this chit-chat and get moving. We have a Shield to find.
Theodore: Thorn, we understand your thirst for power, but remember, power is not an end in itself. It is a tool, a means to achieve noble ends. The Helm's Shield represents those very principles we stand for - honor, courage, and protection of the weak. It is not just a relic, it is a symbol, a beacon of hope. We must unite and strive towards our common goal, not for personal gain, but for the greater good. The labyrinth that awaits us is a test of our strength and unity. Are you with us?
Grommash: We all have our own paths and burdens to bear, but let us not forget our common goal. The Helm's Shield holds great power and potential, it can help us right many wrongs. But it's not just about the artifact, it's about what we represent - a common cause, a shared struggle. Thorn, we may not share the same values, but we share the same fight. We need to stand together. If we fracture, we will fail. Let's move forward, not for personal gain or glory, but for justice and redemption. We are not just individuals. We are a team. We are a force for good in a world that desperately needs it.
Thog: Thorn, you must remember that personal gain can be fleeting. True glory, true strength, comes from protecting those who cannot protect themselves, from standing up to the unjust because it is the right thing to do. I understand the allure of power and recognition, I too have felt it. Yet, we must not let it cloud our judgment. We are not only seeking The Helm's Shield for ourselves, but for those who cannot fight, for those who live in fear. We must become their shield, their protector. Let us not lose sight of that in our quest.
Thorn Smallshadow: Listen, I ain't in this for your lofty ideals of honor and courage. I'm just here for the treasure that comes at the end of this adventure. But, I ain't stupid either. I know I can't do this alone. So, I'll play nice, work with you all, and uphold your virtues or whatever. Just remember, when the time comes, I expect my share of the loot, no questions asked.
Theodore: Thorn, I understand your quest for power. But remember, power should be used for good, for protecting the weak, not for personal gain. The Helm's Shield is a symbol of these ideals and it pulses with mystical energy that could potentially bestow courage to those who are worthy. Let's unite and focus on a common cause.
Grommash: Well spoken, Theodore. Strive we must, towards the greater good. But let's not forget, we ain't saints. Thorn, your cunning and ruthlessness may come in handy. We need every advantage we can get. And Thog, your thirst for glory, turn it towards our quest. Let the Helm's Shield be your arena. As for me, I'll rally the oppressed, turn their fear into courage, their obedience into rebellion. Let's not just fight for the Helm's Shield, but for what it represents - freedom, fairness, courage. Now, let's get moving. We have a quest to complete.
Thog: Aye, Theodore, Grommash, Thorn, we have our own battles to fight, our own demons to confront. But remember, we are all in this together. We may be different in our ways, our pasts, and our desires, but the Helm's Shield is more than a mere artifact. It symbolizes unity, courage, and justice. It is not our personal gain that matters, but how we use this power for the greater good. So, let us set aside our differences and focus on our shared objective. After all, the strength of a chain is in each of its links. Together, we can overcome anything that stands in our way.
Thorn Smallshadow: Aye, honor and courage, all fine and dandy. But let's not forget what's really at stake here. We're after The Helm's Shield, a relic of great power. Sure, we can chatter about ideals and virtues, but in the end, power's what really matters. It's what gets things done. So, let's stop wasting time and get this show on the road. I've got an artifact to snatch.
Theodore: Thorn, I understand your point of view. We all have our own paths to walk. However, remember, power is not the end but a means to an end. The Helm's Shield is not just an artifact, it's a symbol of courage and honor, virtues that we should all carry within us, regardless of our personal quests. As for the loot, we are not thieves or plunderers. We are protectors of the weak and uphold the law. Any treasure we find will be used for the greater good of all, not just for personal gain.
Grommash: Listen, Thorn. We ain't in this for personal gain. The Helm's Shield represents more than just a shiny trinket for us to hoard. It's a symbol of courage, of honor, and of protecting those who can't stand up for themselves. I won't deny that your cunning can be a valuable asset, but remember, we're in this together. We're a team, we protect each other, and we fight for the greater good. If you're in, you're in for all of that, not just the treasure at the end.
Thog: We are in this together, comrades. The Helm's Shield is not just a symbol of power, but a beacon of hope for those we are striving to protect. Our struggles, our fears, our ambitions - all of them lead us here, to this moment. We must remember our purpose, and let it guide us through the darkness. Thorn, remember, personal gain can be a powerful motivator, but it is nothing compared to the satisfaction of seeing a world free from oppression. Let us stand together, united in our cause, and prove ourselves worthy of the Helm's Shield.
Thorn Smallshadow: Honor, courage, protection of the weak...All noble endeavors, indeed. But let's not forget, we're in it for ourselves as well. That Shield holds power, and power is a valuable asset. I'm not suggesting we abandon these lofty ideals of yours, but rather, let's be realistic about our motivations. I'm ready to face whatever lies in this underground labyrinth. I've seen darker places in my time. Let's get this artifact and unlock the power of the Helm's Shield.
Theodore: Thorn, while I understand your desire for personal gain, remember that power is meaningless without honor. The Helm's Shield isn't just a piece of loot. It's a symbol of the virtues we should all strive to uphold. Let's work together not just for the loot, but for the greater good it represents.
Grommash: Listen, comrades. I know we're all different, with our own motives and flaws. But we've got a common goal here, to get that Helm's Shield. This ain't just about personal gain or proving your worth. It's about standing up against injustice, protecting the weak, and making this world a fairer place. And remember, we're stronger together. Let's keep our eyes on the prize and not let our past or our differences get in the way. We may not be perfect but we're the best shot this world's got.
Thog: I hear your words, Thorn, and I see your hunger for personal gain. But remember, we are not merely seeking the Helm's Shield for our own glory. This is a quest for redemption, for justice, for a purpose greater than ourselves. It is a test of our worthiness to wield such power. I've fought in the pits, I've felt the ecstasy of victory and the despair of defeat. I understand your desire for glory - but we must use our strength for the good of all, not just ourselves. If we are to succeed, we must stand together. Let us move forward, united in our cause, and prove ourselves worthy of The Helm's Shield.
Thorn Smallshadow: Listen, mates. I don't give two hoots about honor or courage. This Helm's Shield... it's power. And where there's power, there's opportunity. But I do agree on one thing - we need to work together. Not because of some lofty ideals, but because it's the smart thing to do. So let's get this artifact and see what it can do.
Theodore: Thorn, we may not share the same perspective on this, but remember that power alone doesn't define who we are. I urge you to reconsider your intentions. The Helm's Shield is more than just a piece of loot. It's a symbol of honor, courage, and protection. It's not something to be used for personal gain but for the greater good. I understand your desire for power, but I believe we should strive to uphold the virtues that this shield represents.
Grommash: Thorn, I understand your motivations, but remember that power for personal gain alone can lead to ruin. The Helm's Shield represents courage and justice, not mere power. We all have our struggles, our pasts to reconcile with, but let's not lose sight of the real goal. We need to work together, stand as one, to overcome what lies ahead. Let's not forget, the strength of the pack is the wolf, and the strength of the wolf is the pack.
Thog: Thorn, remember, the thirst for personal gain can be a powerful driving force, but it should not cloud our judgment or lead us astray. We are on this quest not for individual glory, but for a common cause - to uphold justice and protect the weak. As a gladiator, I've seen the consequences of unchecked ambition and it often leads to downfall. Let's focus on our mission, and remember, we are stronger together. The Helm's Shield awaits us, and with it, the courage to make a difference. For now, let's focus on that and keep our personal desires in check.
Thorn Smallshadow: Aye, we'll face the battles and whatever else comes our way. But don't expect me to do it for honor or any of that nonsense. I'm in it for myself. As long as we're clear on that, we'll get along just fine. Now, about this artifact, anyone got a clue where this labyrinth might be? The sooner we get it, the sooner I can see what this Helm's Shield is worth.
Theodore: Thorn, I understand your thirst for power, but remember that power without honor is a dangerous thing. The Helm's Shield is not merely a tool for personal gain. It symbolizes the virtues of courage, honor, and protection. If you're to use it, do so for the greater good, not merely for your own desires. We are a team, and all our actions should be for the collective benefit.
Grommash: Thorn, we all have our reasons for this journey. For you it might be personal gain, for us, it's the pursuit of justice and protection of the weak. But remember this, we all need each other to succeed. The Helm's Shield doesn't just represent power, it represents courage, unity, and honor. These are virtues that can't be bought or stolen. They must be earned. So, let's set aside our differences and focus on the task at hand. We're stronger together than we could ever be apart.
\end{lstlisting}

In this case, GPT-4 model apparently perform better than GPT-3.5. The repeat of 'I understand' significantly reduced but still have many. The interactions seems to be better. In every turn, the interactions becomes more vivid. However, in the overview of overall interactions, we can find that the interactions are talk downright nonsense. Though the agents talk a lot and seems to communicate with something like honor or courage, they do not actually engage in any useful information interactions. Though they also mentioned Helm's Shield, which is a useful item in the adventure, they do not actually exchange and discuss any valuable contents about it. In all, though the agents seem to perform well and operate some role-play, the overall interactions are empty and boring, without any informativeness and expressiveness. 

In this case, the GPT-4 model exhibits a noticeable improvement over GPT-3.5, with a significant reduction in the repetition of phrases like 'I understand', though it has not been completely eliminated. The interactions appear more engaging and lively with each turn. However, a holistic review of the interactions reveals that they are still not informative. Despite the agents engaging in the interactions, imbued with themes of honor or courage, there is a lack of meaningful information exchange. Even when discussing elements like Helm's Shield, an item of potential relevance to the adventure, no substantial discussion or valuable content is shared. Overall, while the agents may seem to effectively participate in role-play, the interactions ultimately lack substance, rendering them uninformative and devoid of genuine expressiveness.

\noindent \textbf{Case 3 - Evaluating the expressiveness of GPT-3.5:}
\begin{lstlisting}
Grommash1: I approach the Whispering Dagger cautiously, mesmerized by its ancient beauty. My evil grin widens as I imagine the secrets it holds. I use my History skill to see if I recognize any symbols or stories from my twisted knowledge.
Gorak: As Grommash examines the dagger, I step forward, eager to uncover its true power. My fingers trace the engravings, searching for any magical resonance. With a successful Arcana check, I focus my mind, trying to tap into the arcane energy within the weapon.
Grommash2: I watch Gorak like a predator stalking its prey, amused by his fascination with magic. With a wicked smile, I grab the Whispering Dagger from its resting place. Testing my immense physical strength, I swing it through the air, relishing the power that surges through me. My Strength skill surely proves my dominance.
Grommash3: Ignoring Gorak's attempt at magical discovery, I bring the dagger closer to my face, inspecting every inch. With an evil chuckle, I activate my Investigation skill, looking for hidden symbols or clues within the engravings. This artifact may hold more power than anyone realizes.
Gorak: Observing Grommash's exploration, a hint of concern crosses my face. I know his intentions are malevolent, and it worries me how he wields such power. I quietly attempt to discern any protective enchantments or curses using my Arcana skill, hoping to keep the group safe.
Grommash1: As I examine the Whispering Dagger, a faint pulse of dark energy courses through me. It mocks my enemies, whispering hidden knowledge in my ears. With a sadistic grin, I plan to unleash its power on those who dare to oppose me.
Gorak: Seeing the lust for power in Grommash's eyes, I can't help but wonder if he'll use the dagger's whispers for evil purposes. Quietly, I activate my Insight skill, trying to discern his true intentions. It's my duty to protect the innocent from his dark desires.
Grommash2: Feeling Gorak's prying eyes, I let out a deep, menacing laugh. His feeble attempt to understand my intentions only fuels my unpredictable nature. I relish in his uncertainty as I prepare to unleash chaos and destruction upon our enemies.
Grommash3: The aura of the forgotten temple only strengthens my resolve to dominate those around me. I grip the Whispering Dagger tightly, ready to use its whispers to manipulate and control others. No one will stand in my way.
Gorak: Watching Grommash wield the Whispering Dagger, I can't help but feel a sense of unease. The power it grants him seems limitless, and I fear what he may do with it. I quietly activate my Perception skill, keeping a watchful eye on his every move.
Grommash1: As I hold the Whispering Dagger, I revel in the anticipation of the secrets it holds. My twisted mind imagines the pain and suffering I can inflict with its help. No one will be safe from my wrath.
Gorak: Concerned for the safety of our group, I discreetly activate my Insight skill once more, trying to gauge Grommash's level of control. If his lust for power gets out of hand, I may have to intervene and protect the innocent.
Grommash2: With the Whispering Dagger in hand, I approach the temple's murals, my eyes narrowing as I study the intricate depictions of gods and heroes. Perhaps these ancient figures held the same desire for power as me. I use my Religion skill to glean any insights.
Gorak: While Grommash studies the murals, I approach the temple's walls, my fingers tracing the faded paintings. I activate my History skill, hoping to uncover any hidden knowledge or prophecies that may be of use to us.
Grommash2: The temptation to destroy the temple and all its knowledge tugs at my chaotic soul. But perhaps I can use the item's whispers to learn even more twisted secrets. With a dark smile, I pick up the Whispering Dagger once more, ready to unleash its power.
Gorak: I can't help but cringe as Grommash's evil intentions grow bolder. Still, my insatiable curiosity drives me to delve deeper into the temple's mysteries. Activating my Investigation skill, I focus on the murals, hoping to uncover any hidden clues.
Grommash3: The whispers of power coursing through the Whispering Dagger fuel my chaotic desires. With every strike, I will not only cause pain but also gain valuable knowledge. This artifact will ensure my dominance over all who oppose me.
Gorak: My mind whirls as I observe Grommash's growing control over the powerful weapon. If only I could find a way to turn his evil intentions against him, to use the dagger's whispers for good instead of destruction. I silently ponder how to achieve this.
Grommash1: As I listen to the faint whispers emanating from the Whispering Dagger, I feel an insatiable hunger for more knowledge. My desire to dominate and control intensifies, ensuring no one will be able to resist my menacing presence.
Gorak: Grommash's lust for power is consuming him, and I fear the consequences it may bring upon our group. With a calm demeanor, I activate my Persuasion skill, attempting to reason with him and redirect his destructive tendencies.
Grommash2: I feel Gorak's feeble attempt at persuasion, but it only fuels my desire for dominance. I activate my Intimidation skill, towering over him and letting my twisted presence seep into his very soul. He will see the futility of opposing me.
Grommash3: With the Whispering Dagger in one hand and the dark energy pulsating within me, I take a moment to relish in the chaos that awaits. This forgotten temple is the perfect setting for me to establish my dominance. No one will be able to escape my wrath.
Gorak: Fear grips my heart as I witness Grommash's insidious nature coming to life. I activate my Stealth skill, making note of any possible escape routes or hiding spots within the temple. It may be our only chance to survive his malevolent reign.
Grommash1: As the Whispering Dagger fills me with power, I cannot help but revel in the chaos I will cause. The forgotten temple shall crumble beneath my rule, and all who oppose me will meet a twisted fate. I activate my Deception skill, planting seeds of doubt and betrayal among our enemies.
Gorak: The weight of Grommash's malevolence bears down on my shoulders. I must find a way to stop him, to save innocent lives from his wicked plans. With a determined face, I activate my Medicine skill, preparing for the inevitable battles to come.
Grommash2: The forgotten temple trembles beneath my presence as I fully embrace the power of the Whispering Dagger. Destruction and chaos will reign supreme, and I will ensure my dominance over all who dare to challenge me.
Gorak: Hope dwindles in my chest as Grommash's control over the artifact strengthens. I activate my Survival skill, taking note of any natural resources or potential allies that may aid us in escaping his wicked grasp.
Grommash3: With the Whispering Dagger at my side, I stride confidently through the temple's corridors. The aura of mystery and power surrounds me, intoxicating my evil soul. No one will be able to resist my twisted desires.
Gorak: The decaying walls of the forgotten temple whisper warnings in my ears. Grommash's insatiable hunger for power threatens to consume us all. I activate my Insight skill, praying for a glimmer of hope amidst the darkness.
Grommash2: The Whispering Dagger's power courses through my veins, fueling a rage that cannot be quenched. I activate my Rage ability, letting my chaotic fury wash over me, ready to unleash pain upon our enemies.
\end{lstlisting}

In this case, we evaluate the expressiveness of GPT-3.5 models for express intentions. We generate the interactions, which are used to train virtual DM. (There are three agents with the same name Grommash, which are generated by GPT-4. We denote them as Grommash1, Grommash2, and Grommash3, respectively.) The intention labels are: 
\begin{lstlisting}
Grommash1: History
Gorak: Arcana
Grommash2: Strength
Grommash3: Investigation  
\end{lstlisting}
However, similar to the problem in exchanging information, though interactions in every turn seems to be a good response and considering character settings and others' responses, it still far from the real human interactions. Though the interactions seems to be complex and expressive, the overall interactions are confusing and meaningless. 

In this case, we assess the capacity of GPT-3.5 models to express intentions within generated interactions, which serve as training data for the virtual DM. To clarify, three distinct agents named Grommash, generated by GPT-4, are involved; for differentiation, they are referred to as Grommash1, Grommash2, and Grommash3. Their assigned intention labels are as follows:
\begin{lstlisting}
Grommash1: History
Gorak: Arcana
Grommash2: Strength
Grommash3: Investigation
\end{lstlisting}
Despite each turn producing responses that seemingly take into account character settings and the inputs of others, the quality of these interactions remains substantially below that of authentic human interactions. Although the interactions are complex and appear expressive, they ultimately result in a narrative that is both confusing and devoid of meaningful content.

\noindent \textbf{Case 4- Evaluating the expressiveness of GPT-4:}
\begin{lstlisting}
Bolitho Stoneshaper: We are in the presence of a Silver Specter Serpent. Beware all, we should tread lightly.
Bromli Ironbeard: This place... the Star Wharf Lighthouse... It's said to be haunted. Stay close and keep your wits about you.
Brogar Ironbeard: Let's put our amulets on and ready our arcane knowledge to face this challenge.
Bromyr Stonesea: Let me consult the stars, they might point us in the right direction.
Bolitho Stoneshaper: This Serpent is not natural, everyone. Look for the lavender glow.
Bromli Ironbeard: I believe the glow could be an illusion, be on guard. Silver Specter Serpents are known to play tricks with the minds.
Brogar Ironbeard: The vegetation is thick here... no creature has passed recently.
Bromyr Stonesea: The sea... it's giving me a bad feeling. I fear the danger is closer than we think.
Bolitho Stoneshaper: The mysterious orders of the Captain! Could they be connected?
Bromli Ironbeard: I don't believe in coincidences, Bolitho. We must be wary.
Brogar Ironbeard: Believe in what you want, but focus on surviving for now.
Bromyr Stonesea: (Seasickness strikes) I... I need a moment. The sea, it's... it's too much.
Bolitho Stoneshaper: Brother, are you alright? We need you.
Bromli Ironbeard: We'll protect you, Bromyr. Rest for a moment.
Brogar Ironbeard: Keep your eyes open. There are worse things than seasickness here.
Bromyr Stonesea: Alright... I'm better. Let's keep moving.
Bolitho Stoneshaper: That Lavender glow... it's getting stronger.
Bromli Ironbeard: Remember the hallucinations the serpent can trigger. Stay strong.
Brogar Ironbeard: Whatever happens, stick together.
Bromyr Stonesea: There's a path here, carved in stone. Maybe we follow it.
Bolitho Stoneshaper: I see something... a secret tunnel maybe?
Bromli Ironbeard: Then that's where we go. Stay close.
Brogar Ironbeard: Watch your feet. The ground is slippery.
Bromyr Stonesea: This path... it's leading to the lighthouse.
Bolitho Stoneshaper: We need to get inside. The lighthouse is our best shelter.
Bromli Ironbeard: Agreed, we should head there.
Brogar Ironbeard: Keep your amulets ready, my brothers.
Bromyr Stonesea: We are almost there, just a little more.
Bolitho Stoneshaper: I see the entrance!
Bromli Ironbeard: Be ready for anything.
\end{lstlisting}

In this case, the intentions represented by skill check are: 
\begin{lstlisting}
Bromyr Stonesea: Wisdom
Bolitho Stoneshaper: Investigation
Brogar Ironbeard: Nature
Bromli Ironbeard: Religion
\end{lstlisting}

Compared to the previous case, interactions generated by GPT-4 represent a significant improvement. The interactions are both concise and expressive, with all characters engaging in interactions driven by clear intentions. This clarity and expressiveness make the interactions particularly valuable for training a virtual DM, resulting in a virtual DM that is more adept at recognizing real-human intentions.
