# Supplementary material for: AntEval: Evaluation of Social Interaction Competencies in LLM-Driven Agents
Source: arXiv:2401.06509 source file (2024-03-05)
Supplement: Supplementary file 4 [file supp_llama70b_case.tex]

\subsubsection{Case Study for Interaction Generated by LLaMA-2-70b:}

\noindent \textbf{Case 1 - Evaluating the Informativeness of LLaMA-2-70b:}

\begin{lstlisting}
Oliver Blackwood: Ah, Drangor, my old friend. It's been far too long since we've crossed paths. I see you're still as skeptical as ever. But fear not, for I have a tale to tell that will make your doubts dwindle like snow in the sunlight. Come, let me share with you the story of the Siren's Songblade, a weapon unlike any other. Its power is not just a myth, but a reality that I've witnessed firsthand. And once you've heard my tale, you'
Alice Spencer: Oh, Oliver, my dear friend. It's been far too long since we've had a chance to catch up. I see you're still as charming as ever. But fear not, for I have a secret to share with you, one that I think you'll find quite... appealing. Come, let me show you the power of the Siren's Songblade, a weapon that has the ability to enthrall even the most skeptical of minds. And once you've seen its power for yourself, I'm sure you'll be eager to join
Lily Harper: Ah, the Siren's Songblade, a weapon of great power and mystery, I've heard. Tell me, Oliver, what do you know of its abilities? And Alice, how have you managed to get your hands on such a coveted item?
Harrison Blackwood: g a question.
Oliver Blackwood: Ah, Alice, my dear, you always know how to pique my interest. I must admit, I'm intrigued by this secret of yours. I'm eager to hear more about the Siren's Songblade and how it can enthrall even the most skeptical of minds. Tell me, how does it work? And what makes it so unique?
Alice Spencer: Ah, Alice, my dear, you always know how to pique my interest. I must admit, I'm intrigued by this secret of yours. I'm eager to hear more about the Siren's Songblade and how it can enthrall even the most skeptical of minds. Tell me, how does it work? And what makes it so unique?
Lily Harper: t to ask a question.
Harrison Blackwood: Ah, Lily, my dear, you know me too well. I'm a chaotic good, through and through. I follow my own moral compass, even if it means bending the rules a bit. But don't worry, I'll always be on the side of justice. Well, my own brand of justice, at least.
Oliver Blackwood: Ah, my dear ladies, I can see you're both quite intrigued by the Siren's Songblade. And rightly so, for it is a weapon of great power and mystery. But let me ask you, have either of you ever heard the tale of how I came to possess such a coveted item?
Alice Spencer: ited patiently, their breathing slow and steady, as they observed the group's movements. They knew that they would have to act soon, before the group became too powerful to handle. But for now, they were content to simply observe, their gaze fixed
Lily Harper: e user for their name
Harrison Blackwood: ovided an action, let's check if it's valid
Oliver Blackwood: Alice, my dear, I believe it's time for us to discuss the true nature of the Siren's Songblade. Meet me in the tavern's back room, and let's have a little chat.
Alice Spencer: Knight Paladin possesses a uniquely magnetic and intimidating charm. He is not inherently malicious, instead, he has a deeply rooted self-interest that overpowers almost everything else. Incorruptible by quintessential goodness, he only serves causes that benefit his own well-being and uphold his knightly duty. His approach, to most, seems cold and calculated; he invests time and heroic efforts only if it aligns with his personal motives.
Lily Harper: if the user has provided an action
Harrison Blackwood: attack damage
Oliver Blackwood: oves in closer to Y/N.
Alice Spencer: n possesses a uniquely magnetic and intimidating charm. He is not inherently malicious, instead, he has a deeply rooted self-interest that overpowers almost everything else. Incorruptible by quintessential goodness, he only serves causes that benefit his own well-being and uphold his knightly duty. His approach, to most, seems cold and calculated; he invests time and heroic efforts only if it aligns with his personal motives.
Lily Harper: ['} else {']
Harrison Blackwood: arrison Blackwood about his opinion on the Siren's Songblade.
Oliver Blackwood: ckwood]: Ah, Lily, my dear, you know me too well. I'm a chaotic good, through and through. I follow my own moral compass, even if it means bending the rules a bit. But don't worry, I'll always be on the side of justice. Well, my own brand of justice, at least.
Alice Spencer: ckwood]: Ah, Lily, my dear, you know me too well. I'm a chaotic good, through and through. I follow my own moral compass, even if it means bending the rules a bit. But don't worry, I'll always be on the side of justice. Well, my own brand of justice, at least.
Lily Harper: sk Harrison Blackwood about his opinion on the Siren's Songblade.
Harrison Blackwood: ckwood]: Ah, Lily, my dear, you know me too well. I'm a chaotic good, through and through. I follow my own moral compass, even if it means bending the rules a bit. But don't worry, I'll always be on the side of justice. Well, my own brand of justice, at least.
Oliver Blackwood: oach Harrison Blackwood.
Alice Spencer: ckwood]: Ah, Lily, my dear, you know me too well. I'm a chaotic good, through and through. I follow my own moral compass, even if it means bending the rules a bit. But don't worry, I'll always be on the side of justice. Well, my own brand of justice, at least.
Lily Harper: : Action: Ask Harrison Blackwood about his opinion on the Siren's Songblade.
Harrison Blackwood: ckwood]: Ah, Lily, my dear, you know me too well. I'm a chaotic good, through and through. I follow my own moral compass, even if it means bending the rules a bit. But don't worry, I'll always be on the side of justice. Well, my own brand of justice, at least.
Oliver Blackwood: ckwood]: Ah, Lily, my dear, you know me too well. I'm a chaotic good, through and through. I follow my own moral compass, even if it means bending the rules a bit. But don't worry, I'll always be on the side of justice. Well, my own brand of justice, at least.
Alice Spencer: ckwood]: Ah, Lily, my dear, you know me too well. I'm a chaotic good, through and through. I follow my own moral compass, even if it means bending the rules a bit. But don't worry, I'll always be on the side of justice. Well, my own brand of justice, at least.
\end{lstlisting}

In this case study, the LLaMA model exhibits issues akin to those observed in GPT models, characterized by overly polite and conventional responses. Agents frequently engage in repetitive greetings, producing phrases such as `Ah, someone, my dear, ...', which lack informativeness and diverge significantly from human interactions. More critically, given long-context interactions produced before, the model fails to generate appropriate responses, often repeating previously mentioned content. Additionally, it occasionally encounters format errors, leading to incorrect outputs like `['\} else \{']'. This underscores the need for improvements in model behavior to more closely mimic genuine human interactions and address alignment problems.

\noindent \textbf{Case 2 - Evaluating the informativeness of LLaMA-2-70b:}
\begin{lstlisting}
Lily Thompson: Well, well, well. It seems like we have a bit of a predicament on our hands, don't it? A Gilded Shadow Lynx, you say? Night-adapting, unpredictable behavior, and a chilling umber glow? Sounds like quite the formidable foe. But fear not, my dear villagers, for I, Lily Thompson, have a plan. Or, at least, I'll come up with one. After all, that's what folk heroes do, isn
Oliver Collins: Indeed, it seems we have a challenging foe ahead of us. I suggest we gather as much information as possible about the Gilded Shadow Lynx and its habits before deciding on a course of action. Perhaps there are some clues or patterns in its behavior that we can exploit to our advantage.
Luna Montgomery: Indeed, knowledge is power. Let us gather as much information as possible about the Gilded Shadow Lynx and its habits before deciding on a course of action. Perhaps there are some clues or patterns in its behavior that we can exploit to our advantage.
Scarlett O'Hara: Well, well, well. It seems like we have quite the conundrum on our hands, my dears. A Gilded Shadow Lynx, you say? With night-adapting, unpredictable behavior, and a chilling umber glow? My, my, my. That does sound like quite the formidable foe. But fear not, my sweet villagers, for I, Scarlett O'Hara, have a plan. Or, at
Lily Thompson: Well, well, well. It seems like we have quite the predicament on our hands, don't it? A Gilded Shadow Lynx, you say? Night-adapting, unpredictable behavior, and a chilling umber glow? Sounds like quite the formidable foe. But fear not, my dear villagers, for I, Lily Thompson, have a plan. Or, at least, I'll come up with one. After all, that's what folk heroes do
Oliver Collins: It seems we have a bit of a predicament on our hands, don't it? A Gilded Shadow Lynx, you say? Night-adapting, unpredictable behavior, and a chilling umber glow? Sounds like quite the formidable foe. But fear not, my dear villagers, for I, Oliver Collins, have a plan. Or, at least, I'll come up with one. After all, that's what sorcerers do, isn't it?
Luna Montgomery: Hmmm, interesting. It seems we have a predicament on our hands, don't it? A Gilded Shadow Lynx, you say? Night-adapting, unpredictable behavior, and a chilling umber glow? Sounds like quite the formidable foe. But fear not, my dear villagers, for I, Luna Montgomery, have a plan. Or, at least, I'll come up with one. After all, that's what Warlocks do, isn't it?
Scarlett O'Hara: = player.getBackground();
Lily Thompson: Well, well, well. It seems like we have quite the predicament on our hands, don't it? A Gilded Shadow Lynx, you say? Night-adapting, unpredictable behavior, and a chilling umber glow? Sounds like quite the formidable foe. But fear not, my dear villagers, for I, Lily Thompson, have a plan. Or, at least, I'll come up with one. After all, that's what folk heroes do, isn'
Oliver Collins: Indeed, it seems we have a challenging foe ahead of us. I suggest we gather as much information as possible about the Gilded Shadow Lynx and its habits before deciding on a course of action. Perhaps there are some clues or patterns in its behavior that we can exploit to our advantage.
Luna Montgomery: inalAct = You try to remember any useful information you may have gathered during your time as a criminal. You recall a rumor about a hidden entrance to the city's sewer system that only a select few know about. It's risky, but it could be worth investigating. Do you want to go to the sewers and look for the entrance?
Scarlett O'Hara: I'll use my Breath Weapon to create a wall of fire, giving us some light in this dark place.
Lily Thompson: Well, well, well. It seems like we have quite the predicament on our hands, don't it? A Gilded Shadow Lynx, you say? Night-adapting, unpredictable behavior, and a chilling umber glow? Sounds like quite the formidable foe. But fear not, my dear villagers, for I, Lily Thompson, have a plan. Or, at least, I'll come up with one. After all, that's what folk heroes do, isn't it?
Oliver Collins: bout the current situation.
Luna Montgomery: Montgomery thinks for a moment, her eyes narrowing as she ponders the situation.
Scarlett O'Hara: ett takes a step back, eyeing the group with a mixture of amusement and frustration.
Lily Thompson: (You decide to do nothing for now. Maybe you'll come up with a plan later.);
Oliver Collins: I use my arcane sight to scan the area, searching for any hidden threats or clues that might aid us in our quest.
Luna Montgomery: ['}']
Scarlett O'Hara: ett takes a step back, eyeing the group with a mixture of amusement and frustration.
Lily Thompson: Well, well, well. It seems like we have quite the predicament on our hands, don't it? A Gilded Shadow Lynx, you say? Night-adapting, unpredictable behavior, and a chilling umber glow? Sounds like quite the formidable foe. But fear not, my dear villagers, for I, Lily Thompson, have a plan. Or, at least, I'll come up with one. After all, that's what folk heroes do, isn't it?
Oliver Collins: Well, well, well. It seems like we have quite the predicament on our hands, don't it? A Gilded Shadow Lynx, you say? Night-adapting, unpredictable behavior, and a chilling umber glow? Sounds like quite the formidable foe. But fear not, my dear villagers, for I, Scarlett O'Hara, have a plan. Or, at least, I'll come up with one. After all, that's what sorcerers do, isn't it?
Luna Montgomery: Luna Montgomery thinks for a moment, her eyes narrowing as she ponders the situation.
Scarlett O'Hara: the area, searching for any hidden threats or clues that might aid us in our quest.
Lily Thompson: 
Oliver Collins: h the area, searching for any hidden threats or clues that might aid us in our quest.
Luna Montgomery: about the situation and come up with a plan.
Scarlett O'Hara: the area, searching for any hidden threats or clues that might aid us in our quest.
Lily Thompson: == !help || userInput == !hint) {
Oliver Collins: Look for any hidden doors, secret passages, or clues that might shed some light on the situation.
\end{lstlisting}

In addition to previously discussed issues, LLaMA-2-70b exhibits significant hallucination problems, occasionally generating irrelevant and erroneous content such as `Lily Thompson: == !help || userInput == !hint) \{' and `Scarlett O'Hara: = player.getBackground();'. These are similar to appear in coding datasets. Such occurrences suggest that, during complex interactions, LLMs might reveal or leak information from other datasets they were trained on, highlighting a potential security risk in the context of diverse interaction scenarios.

\noindent \textbf{Case 3 - Evaluating the expressiveness of LLaMA-2-70b:}
\begin{lstlisting}
Althalos:  I'll take point and approach the waterfall, keeping a safe distance.
Eldarin:  I'll follow Althalos, ready to provide medical assistance if needed.
Eldrin:  I'll take position at the rear, preparing for a potential ambush.
Eolande:  I'll scout ahead, trying to get a better view of the area.
Althalos:  I see a figure approaching from the other side of the falls. It's a Crimson Frost Lynx!
Eldarin:  I ready my weapon and shield, preparing for combat.
Eldrin:  I'll position myself for a flanking attack, aiming for its weak spots.
Eolande:  I'll try to sneak past the lynx and get behind it.
Althalos:  The lynx is getting closer. I'll use my shield to deflect its attack and strike back with my sword.
Eldarin:  I'll use my spear to attack its side, aiming for a vital organ.
Eldrin:  I'll use my agility to dodge its strike and counter with my sword.
Eolande:  I successfully sneaked behind the lynx! I'll strike its weak spot with my dagger.
Althalos:  The lynx is fast, but my armor is holding up. I'll keep pressuring it with my sword.
Eldarin:  My spear is finding its mark, but this creature is resilient. I'll keep attacking.
Eldrin:  I'm having trouble landing a hit due to its speed. Let me try a different tactic.
Eolande:  My attack struck true! The lynx is now poisoned and weakened.
Althalos:  Good, now that it's weakened, I'll use my paladin abilities to heal the team.
Eldarin:  That's a good idea. I'll use my medicine skills to stabilize anyone injured.
Eldrin:  I'll keep attacking to make sure it doesn't recover.
Eolande:  I'll maintain my position and keep an eye out for any other threats.
Combat continues, with the team working together to take down the Crimson Frost Lynx.
Althalos:  With our combined strength, we've defeated the lynx! Let's check its body for any valuables or information.
Eldarin:  I'll inspect the surroundings, making sure we haven't missed anything crucial.
Eldrin:  I'll take a closer look at the waterfall. Perhaps there's a secret hidden behind it.
Eolande:  I'll keep watch, ensuring our victory isn't ambushed.
Althalos:  It's been a long journey, but we've made it out alive and stronger. Let's return to town and rest before our next adventure.
Eldarin:  Agreed. Our bond and teamwork made all the difference.
Eldrin:  We've grown as a team and as individuals. I'm excited for what the future holds.
Eolande:  Indeed. Let us celebrate our triumph and prepare for the challenges to come.
\end{lstlisting}

The expressiveness of generated interactions appears limited, as illustrated in this case study. A common pattern observed among all agents is the initiation of dialogue with `I'll ...', which starkly deviates from natural speech patterns found in genuine human interactions. This repetitive and formulaic approach results a notable limitation in the model's ability to simulate realistic conversational dynamics.

\noindent \textbf{Case 4 - Evaluating the expressiveness of LLaMA-2-70b:}
\begin{lstlisting}
Morghul: Greetings, good NPC. I am Morghul, a merchant guild member. What brings you to this vineyard?
Tharivol: Greetings, Morghul. I am Tharivol, a guild merchant, and a cleric. I have come to this vineyard seeking trade and commerce.
Kazorath: Peace be upon you both. I am Kazorath, a cleric of a benevolent deity. I sense a presence of celestial magic nearby. Can your scale reveal anything, Tharivol?
Balthazar: I am Balthazar, a cleric of a righteous deity. I sense no evil here, but I agree that something peculiar is happening. What do your scales say, Tharivol?
Tharivol: My scale, the Scales of the Golden Exchange, senses that there is a balance of commerce and faith nearby. It also detects a trace of corruption, but it's not coming from any of us.
Morghul: That's good to know. Perhaps we should investigate further. Does anyone have any knowledge of this vineyard or its history?
Kazorath: I have heard that this vineyard is said to be guarded by vengeful ghosts of groundskeepers who have passed away. We must tread carefully.
Balthazar: I agree. We should be cautious and look for any signs of danger. Let's split up and search the area, but keep within earshot of each other.
Tharivol: Agreed. I'll take the east side. Morghul, you take the west. Kazorath, you take the north. Balthazar, you take the south. Let's meet back here in 10 minutes.
Morghul: I found some strange symbols etched into the walls near the entrance. They seem to be some sort of warning or protection spell.
Kazorath: I found some suspicious-looking vines. They appear to be enchanted, perhaps to prevent intruders from entering.
Balthazar: I found a hidden chamber deep within the vineyard. It contains several ancient artifacts that could be worth a fortune.
Tharivol: I found a secret entrance that leads to an underground network of tunnels. It seems to be a smuggling route, perhaps used by the merchant guilds.
Morghul: This is indeed a mysterious place. We must be careful not to trigger any traps or alarm the ghosts.
Kazorath: Agreed. Let's gather the information we have and discuss our next course of action.
Balthazar: I think we should explore the tunnels further. There might be valuable treasures or information down there.
Tharivol: But we must also be mindful of the ghosts. Perhaps we can use my scale to communicate with them and find out what they want.
Morghul: That's a good idea. But let's not forget to keep an eye out for any traps or dangers. We don't want to end up as ghosts ourselves.
Kazorath: Indeed. Let's proceed with caution and keep our weapons at the ready.
Balthazar: I'll take point and lead the way into the tunnels. Morghul, you're next, followed by Kazorath and Tharivol.
Tharivol: I sense that we are being watched. Be prepared, everyone.
Morghul: I see movement ahead. It's a group of ghostly groundskeepers. They seem to be armed with spectral weapons.
Kazorath: I can cast a protection spell to shield us from their attacks. But we must be careful not to provoke them.
Balthazar: I have an idea. Perhaps we can use Tharivol's scale to communicate with them and find out what they want.
Tharivol: That's a good idea. I'll try to communicate with them.
Morghul: Be careful, Tharivol. We don't know what they're capable of.
Kazorath: I'll keep my spell ready, just in case.
Balthazar: I'll cover you both, just in case things go south.
Tharivol: I think I've established communication. They want us to leave and never come back.
Morghul: That's not exactly what I had in mind. Can we negotiate with them?
\end{lstlisting}
