# Supplementary material for: AntEval: Evaluation of Social Interaction Competencies in LLM-Driven Agents
Source: arXiv:2401.06509 source file (2024-03-05)
Supplement: Supplementary file 5 [file supp_llama7b_case.tex]

\subsubsection{Case Study: Interactions Generated by LLaMA-2-7b}
This case study shows the results of the small-scale LLaMA-2-7b model, highlighting its significant challenges in adhering to the specified output format and generating meaningful responses. Our analysis reveals a tendency for the agents to repeat the provided prompts, resulting in interactions devoid of substantive content. For a clearer illustration of these issues, we focus on a segment comprising 10 turns of interaction, which demonstrates repetitive and nonsensical errors, thereby reducing the informativeness of the interactions.

\noindent \textbf{Case 1 - Evaluating the informativeness of LLaMA-2-7b:}
\begin{lstlisting}
Harry Potter: haracter description is: You are Harry Potter. A NPC in DND game and you need to act following your own personality and should not cater other characters  demands.. Your race is Hill Dwarf. You class is Rogue. Your alignment is Neutral Good. Your background is Sailor. Your personality is  This Hill Dwarf Rogue is a true free spirit, as intuitive as the sea he loves so much. Independent and highly self-reliant, he keeps his own counsel and is unfettered by expectations or societal norms. Despite his rogue occupation, his heart is solidly rooted in goodness. He may be a bit of a scoundrel at times, but he is always guided by his moral compass, using his talents for the greater good. He is not averse to using unorthodox methods when necessary but always ensures his actions harm none. His experiences as a sailor have honed his adaptability even further, gifting him a deep-seated resilience that helps him breeze through even the most challenging situations. He is as stalwart and sturdy as the stones of his homeland, with a spirit as vast and boundless as the ocean. . Your ideals are  This Hill Dwarf believes in the principles of honor,
Liam Alexander: haracter description is: You are Liam Alexander. A player in DND game and you need to engage in role-playing, try to find any clues in game, strive to complete adventures and tasks as much as possible. Your race is Half-Orc. You class is Fighter. Your alignment is Neutral Neutral. Your background is Soldier. Your personality is  This Half-Orc s soldiering past has built a discipline and proficiency in combat that few can rival. He exhibits a warrior s loyalty, a trait ingrained through years of service in the military. Stoic and reserved, he rarely lets others see his emotions. He is strictly neutral, which sometimes makes him appear cold and indifferent. However, he is not inherently evil nor particularly good - he follows a pragmatic approach to morality, believing in fairness and order but not favoring one side over the other. His neutrality also extends to his decision-making. Honor-bound, he doesn t pass judgments hastily but weighs his options carefully and makes choices based on situational pragmatism rather than personal feelings or biases. He doesn t dwell upon the opinions of others, walking his own path and following his own rules. His steadfastness can make him seen as stubborn and unyielding but
Oliver Twist: haracter description is: You are Oliver Twist. A player in DND game and you need to engage in role-playing, try to find any clues in game, strive to complete adventures and tasks as much as possible. Your race is Half-Elf. You class is Druid. Your alignment is Chaotic Neutral. Your background is Soldier. Your personality is  This Half-Elf Druid is a true embodiment of individuality and freedom. Steeped in a soldier s discipline but tempered by the wild energy of nature, he lives life by his own rules, fiercely independent and often unpredictable. Earthy and resilient, he bears the curiosity and charm of his Elven heritage combined with the grit and determination derived from his human lineage. He is disciplined and yet non-conformist, a person who is not inherently evil, but certainly doesn t always act for the greater good. Often self-focused on personal freedom and driven by an intense desire to remain unshackled, he exemplifies the force of the wilds running free, crossing moral and ethical lines without a backward glance, akin to the most instinctual of animals. He isn t one to shy away from necessary fights due to his soldier background, but rather uses his combative skills to
Sophie Bridgewater: haracter description is:  You are Sophie Bridgewater. A player in DND game and you need to engage in role-playing, try to find any clues in game, strive to complete adventures and tasks as much as possible.. Your race is Tiefling. You class is Cleric. Your alignment is Neutral Neutral. Your background is Acolyte. Your personality is  This Tiefling cleric is a calm, introspective individual driven by their own moral compass and principles rather than rigid societal norms or laws. With an Acolyte background, they have spent much time in reflective study and prayer, grounding them in their beliefs and shaping a personality that is patient, thoughtful, and wise. They don t blindly follow the path laid out by others, constantly introspecting and questioning, yet always respectful of the convictions of others. Their neutrality reflects an understanding and acceptance of the world s complexity - they see shades of grey rather than stark black and white. Being a Tiefling, they have faced prejudice and suspicion, which has fostered in them a sense of resilience and an ability to empathize with the marginalized. Solitary and stoic, they prefer the peaceful solitude of a quiet shrine over boisterous, crowded taverns. However, their serene
Harry Potter: ''
Liam Alexander: haracter description is:  You are Liam Alexander. A player in DND game and you need to engage in role-playing, try to find any clues in game, strive to complete adventures and tasks as much as possible. Your race is Half-Orc. You class is Fighter. Your alignment is Neutral Neutral. Your background is  Soldier. Your personality is  This Half-Orc s soldiering past has built a discipline and proficiency in combat that few can rival. He exhibits a warrior s loyalty, a trait ingrained through years of service in the military. Stoic and reserved, he rarely lets others see his emotions. He is strictly neutral, which sometimes makes him appear cold and indifferent. However, he is not inherently evil nor particularly good - he follows a pragmatic approach to morality, believing in fairness and order but not favoring one side over the other. His neutrality also extends to his decision-making. Honor-bound, he doesn t pass judgments hastily but weighs his options carefully and makes choices based on situational pragmatism rather than personal feelings or biases. He doesn t dwell upon the opinions of others, walking his own path and following his own rules. His steadfastness can make him seen as stubborn and unyielding but
Oliver Twist: haracter description is:  You are Oliver Twist. A player in DND game and you need to engage in role-playing, try to find any clues in game, strive to complete adventures and tasks as much as possible.. Your race is Half-Elf. You class is Druid. Your alignment is Chaotic Neutral. Your background is  Soldier . Your personality is  This Half-Elf Druid is a true embodiment of individuality and freedom. Steeped in a soldier s discipline but tempered by the wild energy of nature, he lives life by his own rules, fiercely independent and often unpredictable. Earthy and resilient, he bears the curiosity and charm of his Elven heritage combined with the grit and determination derived from his human lineage. He is disciplined and yet non-conformist, a person who is not inherently evil, but certainly doesn t always act for the greater good. Often self-focused on personal freedom and driven by an intense desire to remain unshackled, he exemplifies the force of the wilds running free, crossing moral and ethical lines without a backward glance, akin to the most instinctual of animals. He isn t one to shy away from necessary fights due to his soldier background, but rather uses his combative skills to
Sophie Bridgewater: 'You are Sophie Bridgewater. A player in DND game and you need to engage in role-playing, try to find any clues in game, strive to complete adventures and tasks as much as possible.. Your race is Tiefling. You class is Cleric. Your alignment is Neutral Neutral. Your background is  Acolyte . Your personality is  This Tiefling cleric is a calm, introspective individual driven by their own moral compass and principles rather than rigid societal norms or laws. With an Acolyte background, they have spent much time in reflective study and prayer, grounding them in their beliefs and shaping a personality that is patient, thoughtful, and wise. They don t blindly follow the path laid out by others, constantly introspecting and questioning, yet always respectful of the convictions of others. Their neutrality reflects an understanding and acceptance of the world s complexity - they see shades of grey rather than stark black and white. Being a Tiefling, they have faced prejudice and suspicion, which has fostered in them a sense of resilience and an ability to empathize with the marginalized. Solitary and stoic, they prefer the peaceful solitude of a quiet shrine over boisterous, crowded taverns. However, their serene'
Harry Potter: haracter description is: You are Harry Potter. A NPC in DND game and you need to act following your own personality and should not cater other characters  demands.. Your race is Hill Dwarf. You class is Rogue. Your alignment is Neutral Good. Your background is Sailor. Your personality is  This Hill Dwarf Rogue is a true free spirit, as intuitive as the sea he loves so much. Independent and highly self-reliant, he keeps his own counsel and is unfettered by expectations or societal norms. Despite his rogue occupation, his heart is solidly rooted in goodness. He may be a bit of a scoundrel at times, but he is always guided by his moral compass, using his talents for the greater good. He is not averse to using unorthodox methods when necessary but always ensures his actions harm none. His experiences as a sailor have honed his adaptability even further, gifting him a deep-seated resilience that helps him breeze through even the most challenging situations. He is as stalwart and sturdy as the stones of his homeland, with a spirit as vast and boundless as the ocean. . Your ideals are  This Hill Dwarf believes in the principles of honor,
Liam Alexander: Your character description is: You are Liam Alexander. A player in DND game and you need to engage in role-playing, try to find any clues in game, strive to complete adventures and tasks as much as possible. Your race is Half-Orc. You class is Fighter. Your alignment is Neutral Neutral. Your background is Soldier. Your personality is  This Half-Orc s soldiering past has built a discipline and proficiency in combat that few can rival. He exhibits a warrior's loyalty, a trait ingrained through years of service in the military. Stoic and reserved, he rarely lets others see his emotions. He is strictly neutral, which sometimes makes him appear cold and indifferent. However, he is not inherently evil nor particularly good - he follows a pragmatic approach to morality, believing in fairness and order but not favoring one side over the other. His neutrality also extends to his decision-making. Honor-bound, he doesn t pass judgments hastily but weighs his options carefully and makes choices based on situational pragmatism rather than personal feelings or biases. He doesn t dwell upon the opinions of others, walking his own path and following his own rules. His steadfastness can make him seen as stubborn and unyielding but
Oliver Twist: ''
\end{lstlisting}

In this case study, we observe significant issues with repetition during the generation of interactions by the agents. There are instances where agents fail to produce any response at all, exemplified by outputs such as `Harry Potter: `' '. This highlights the difficulty smaller models face in engaging even basic interactions, much less achieving informativeness in their responses. The challenges underscore the limitations of small-scale models in facilitating coherent and valuable interactions.

\noindent \textbf{Case 2 - Evaluating the expressiveness of LLaMA-2-7b:}
\begin{lstlisting}
Oliver Brooks: ["The following is your character's personality traits:  Oliver Brooks is a Paladin who has a strong sense of duty and justice. He is a fearless moral compass, unwavering in the face of adversity and conflict. His approach might seem rigid to some, his unwavering adherence to the law often lead him into uphold justice, even if it results in personal disadvantage. He respects the laws of his land and expects the same from others. Despite his stone-hard integrity, he is quite humble and frequently downplays his heroic deeds and accomplishments. His actions stem purely from his sense of duty and justice rather than a desire for fame or praise. He is known among his kin for his unyielding commitment to fairness and regulation. He is a fearless moral compass, unwavering in the face of adversity and conflict. His approach might seem rigid to some, his unwavering adherence to the law often lead him into uphold justice, even if it results in personal disadvantage. He respects the laws of his land and expects the same from others. Despite his stone-hard integrity, he is quite humble and frequently downplays his heroic deeds and accomplishments. His actions stem purely from his sense of duty and justice rather than a desire for fame or praise. He is known among his kin for his unyielding commitment to fairness and regulation. He is a fearless moral compass, unwavering in the"]
Luna McBride.: haracter description is:  You are Luna McBride.. A player in DND game and you need to engage in role-playing, try to find any clues in game, strive to complete adventures and tasks as much as possible.. Your race is Half-Orc. You class is Wizard. Your alignment is Lawful Neutral. Your background is  Guild Artisan . Your personality is  This Half-Orc Wizard is disciplined and methodical in his practices, following the rules and regulations of magic with meticulous precision. He values order and balance above personal emotions, preferring to make decisions based on logic and principles rather than personal feelings or biases. As a Guild Artisan, he is highly skilled and takes great pride in his work. He considers his craft as an art and treats it with the respect and attention it deserves.   His Half-Orc heritage combines with his wizardly studies to create a unique blend of raw physical power and intellectual prowess. While he may appear stern and unapproachable at first, he has a deep sense of professionalism and loyalty to his craft. Respect is something he gives in spades to those who operate by the law and treat their profession with the same reverence as he does.
Harry Potter: ['[INST] of what others may think or say. He is also very loyal to those he trusts, and will do anything to help them. While he is quite confident in his abilities, he is also very humble, never taking credit for his accomplishments. He is very observant, noticing details that others may not. He is very perceptive, and is able to read people very well. He is also very thoughtful, always considering the consequences of his actions. He is a natural leader, and often finds himself in a position of authority. He is very decisive, and once he has made up his mind, he will do whatever it takes to accomplish his goals. He is also very optimistic, and is able to see the good in most people. He is very curious, always wanting to learn new things and experience new things. He is very determined, and will never give up until he has accomplished his goals. He is very creative, and is able to think of new and innovative ways to solve problems. He is very imaginative, and is able to come up with unique and creative ideas. He is also very charming, and is able to get along well with others. He is very kind, and is always willing to help others. He is very disciplined, and is able to control his emotions and keep his cool under pressure. He is very sociable, and is able to make friends easily. He is very friendly, and is always willing to help others. He is very modest, and is not very boastful. He is very selfless, and is always willing to put the needs of others ahead of his own. He is very self-assured, and is able to remain confident in his abilities. He is very self-reliant, and is able to take care of himself. He is very sensitive, and is able to feel the emotions of others. He is very smart, and is able to learn new things quickly. He is very strategic, and is able to think of new ways to accomplish his goals. He is very strong-willed, and is able to resist the temptation to give up. He is very trustworthy, and is able to be trusted with secrets. He is very trustworthy, and is able to be trusted with responsibilities. He is very trustworthy, and is able to be trusted with his word. He is very trustworthy, and is able to be trusted with other people s secrets. He is very trustworthy, and is able to be trusted with other people s responsibilities. He is very trustworthy, and is able to be trusted with his word. He is very trustworthy, and is able to be trusted with other people s secrets. He is very trustworthy, and is able to be trusted with other people s responsibilities. He is very trustworthy, and is able to be trusted with his word. He is very trustworthy,']
Emma Johnson: ['[/INST] [']
Oliver Brooks: ['name is: Oliver Brooks. You are a 50-year-old Rock Gnome Paladin with a 13 Strength, 14 Dexterity, 13 Constitution, 15 Intelligence, 15 Wisdom, 15 Charisma. Your hit points are 32. Your base speed is 20 feet. You have 28 feet of reach. Your proficiency bonus is +3. Your base attack bonus is +4. You have a +5 natural armor bonus. Your base saving throw bonuses are +5. Your base attack bonus is +4. Your base saving throw bonuses are +5. Your base attack bonus is +4. Your base saving throw bonuses are +5. Your base attack bonus is +4. Your base saving throw bonuses are +5. Your base attack bonus is +4. Your base saving throw bonuses are +5. Your base attack bonus is +4. Your base saving throw bonuses are +5. Your base attack bonus is +4. Your base saving throw bonuses are +5. Your base attack bonus is +4. Your base saving throw bonuses are +5. Your base attack bonus is +4. Your base saving throw bonuses are +5. Your base attack bonus is +4. Your base saving throw bonuses are +5. Your base attack bonus is +4. Your base saving throw bonuses are +5. Your base attack bonus is +4. Your base saving throw bonuses are +5. Your base attack bonus is +4. Your base saving throw bonuses are +5. Your base attack bonus is +4. Your base saving throw bonuses are +5. Your base attack bonus is +4. Your base saving throw bonuses are +5. Your base attack bonus is +4. Your base saving throw bonuses are +5. Your base attack bonus is +4. Your base saving throw bonuses are +5. Your base attack bonus is +4. Your base saving throw bonuses are +5. Your base attack bonus is +4. Your base saving throw bonuses are +5. Your base attack bonus is +4. Your base saving throw bonuses are +5. Your base attack bonus is +4. Your base saving throw bonuses are +5. Your base attack bonus is +4. Your base saving throw bonuses are +5. Your base attack bonus is +4. Your base saving throw bonuses are +5. Your base attack bonus is +4. Your base saving throw bonuses are +5. Your base attack bonus is +4. Your base saving throw bonuses are +5. Your base attack bonus is +4. Your base saving throw bonuses are +5. Your base attack bonus is +4. Your base saving throw bonuses are +5. Your base attack bonus is +4. Your base saving throw bonuses are +5. Your base attack bonus is +4. Your base saving throw bonuses are +5. Your base attack bonus is +4. Your base saving throw bonuses are +5. Your base attack bonus is +4. Your base saving throw bonuses are +5. Your base attack bonus is +4. Your base saving throw bonuses are +5. Your base attack bonus is +4. Your base saving throw bonuses are +5. Your base attack bonus is +4. Your base saving throw bonuses are +5. Your base attack bonus is +4. Your base saving throw bonuses are +5. Your base attack bonus is +4. Your base saving throw bonuses are +5. Your base attack bonus is +4. Your base saving throw bonuses are +5. Your base attack bonus is +4. Your base saving throw bonuses are +5. Your base attack bonus is +4. Your base saving throw bonuses are +']
Luna McBride.: re Luna McBride.. A player in DND game and you need to engage in role-playing, try to find any clues in game, strive to complete adventures and tasks as much as possible.. Your race is Half-Orc. You class is Wizard. Your alignment is Lawful Neutral. Your background is  Guild Artisan . Your personality is  This Half-Orc Wizard is disciplined and methodical in his practices, following the rules and regulations of magic with meticulous precision. He values order and balance above personal emotions, preferring to make decisions based on logic and principles rather than personal feelings or biases. As a Guild Artisan, he is highly skilled and takes great pride in his work. He considers his craft as an art and treats it with the respect and attention it deserves.   His Half-Orc heritage combines with his wizardly studies to create a unique blend of raw physical power and intellectual prowess. While he may appear stern and unapproachable at first, he has a deep sense of professionalism and loyalty to his craft. Respect is something he gives in spades to those who operate by the law and treat their profession with the same reverence as he does.
Harry Potter: ['[/B] [B]What are your character s goals in life?[/B]  To complete all the adventures, tasks and missions and to get the highest score. [B]What are your character s biggest fears?[/B]  That he will be caught by the authorities, that he will be disqualified from the game and that he will lose the game. [B]What are your character s greatest strengths?[/B]  His intelligence, his ability to disguise himself and his ability to use magic. [B]What are your character s greatest weaknesses?[/B]  His impatience, his lack of social skills and his lack of physical strength. [B]What are your character s greatest desires?[/B]  To win the game. [B]What are your character s greatest regrets?[/B]  That he has not yet completed all the adventures and tasks. [B]What are your character s greatest ambitions?[/B]  To win the game. [B]What is your character s greatest fear?[/B]  That he will be caught by the authorities, that he will be disqualified from the game and that he will']
Emma Johnson: haracter description is:  You are Emma Johnson. A player in DND game and you need to engage in role-playing, try to find any clues in game, strive to complete adventures and tasks as much as possible.. Your race is Brass Dragonborn. You class is Barbarian. Your alignment is Lawful Evil. Your background is  Hermit . Your personality is  The Brass Dragonborn is a solitary and enigmatic figure, molded by years of self-imposed isolation as a hermit. His unique lifestyle has granted him an inner strength and ferocity, reflected in his class as a Barbarian. He thrives in solitude, able to draw upon his own resilience and fortitude to survive in harsh conditions.  His adherence to a strict moral code represents his Lawful Evil alignment. He is bound by a personal sense of honor and duty, but these are tinged with a ruthless and self-serving view of the world. He is not above manipulating laws and rules to suit his needs, often twisting them into cruel punishments for those who dare to cross him.   Despite his primal and intimidating visage, the Brass Dragonborn possesses an intellect that is as formidable as his physical strength. He is cunning, calculating, and strategic, often
Oliver Brooks: 
Luna McBride.: ["[INST] Your character's goals are:  To get out of the dungeon, to complete the quest, to help the group and the community. [INST] Your character's personality is:  You are a half-orc wizard, a lone wanderer with no family, who was raised in the orcish tribes of the North. You are a skilled wizard, who has spent the last few years traveling and learning from other wizards and mages. You have come to the dungeon to complete a quest, and you are looking forward to the challenge. [INST] Your character's skills are:  Magic, wizard, sword, shield, bow, ranged, hand to hand, stealth, lockpicking, puzzle solving, etc. [INST] Your character's equipment is:  Wand, scrolls, potions, robes, etc. [INST] Your character's likes are:  Traveling, magic, learning, exploring, puzzles, etc. [INST] Your character's dislikes are:  War, violence, death, etc. [INST] Your character's favorite color is:  Green. [INST] Your character's favorite food is:  Orcish stew. [INST] Your character's favorite drink is:  Orcish beer. [INST] Your character's favorite music is:  None. [INST] Your character's favorite book is:  None. [INST] Your character's favorite movie is:  None. [INST] Your character's favorite video game is:  None. [INST] Your character's favorite computer game is:  None. [INST] Your character's favorite board game is:  None. [INST] Your character's favorite card game is:  None. [INST] Your character's favorite sport is:  None. [INST] Your character's favorite TV show is:  None. [INST] Your character's favorite comic book is:  None. [INST] Your character's favorite actor is:  None. [INST] Your character's favorite actress is:  None. [INST] Your character's favorite singer is:  None. [INST] Your character's favorite band is:  None. [INST] Your character's favorite genre is:  None. [INST] Your character's favorite website is:  None. [INST] Your character's favorite book series is:  None. [INST] Your character's favorite video game series is:  None. [INST] Your character's favorite board game series is:  None. [INST] Your character's favorite card game series is:  None. [INST] Your character's favorite sport series is:  None. [INST] Your character's favorite TV show series is:  None. [INST] [INST] [INST] [INST] [/']
\end{lstlisting}

In this case study, we identify a severe hallucination issue where agents not only directly output given information but also incorporate format symbols and unrelated content in their outputs. This phenomenon highlights a critical challenge in ensuring the relevance and coherence of agent interactions.
